# Supplementary material for: Few-Step Boltzmann Generators via Scalable Likelihood Flow Maps
Source: arXiv:2606.29110 source file (2026-11-03)
Supplement: Supplementary file 1 [file extension_scallop.tex]

\section{Extending and Connecting SCALLOP to Related Works}\label{app:sec:scallop=extension}

\subsection{Extending SCALLOP to Continuous-time SMC}\label{app:sec:scallop-smc}

\paragraph{Sequential Boltzmann Generator with SMC.}
\cite{tan2026scalableequilibriumsamplingsequential} proposes to scaling a trained Boltzmann Generator, parameterized as a normalizing flow, at inference time through continuous-time Sequential Monte Carlo, namely SBG-SMC. We first review SBG-SMC with an abuse to notations that consistent to our work.
Let $p^\theta$ the trained normalizing flow as a proposal distribution and $\pi(x)\propto \exp(-U(x))$ the Boltzmann distribution that would like to sample from. SBG-SMC proposes to interpolating the proposal and target distribution in logarithm space, reading as
\begin{align}
    V_\tau(x)=-(1-\tau)\log p^\theta(x)+\tau U(x),
\end{align}
for $\tau\in[0,1]$, which define a sequence of distributions $q_\tau(x)\propto\exp(-V_\tau(x))$. According to Jarzynski's Equality \citep{Jarzynski_1997}, let $(x_\tau,w_\tau)$ solve the following coupled system of SDE and ODE:
\begin{align}
    \dd x_\tau&= -\epsilon_\tau\nabla V_\tau(x_\tau)\dd\tau + \sqrt{2\epsilon_\tau}\dd W_\tau,\\
    \dd\log w_\tau&=-\partial_\tau V_\tau(x_\tau)\dd \tau,\quad\text{with }x_0\sim p^\theta\text{ and }\log w_0=0,
\end{align}
then for any observable $O$,
\begin{align}
    \int q_\tau(x)O(x)\dd x= \frac{\mathbb{E}[w_\tau O(x_\tau)]}{\mathbb{E}[w_\tau]},
\end{align}
where the expectations in the RHS of the above equality is over the SDE. Pseudo code is provided in \Cref{alg:SBG_sampling}.

\begin{algorithm}
\caption{SBG-SMC Sampling}
\label{alg:SBG_sampling}
\begin{algorithmic}[1]
\Require \# particles $K$, \# annealed distributions $T$, Energy annealing schedule $V_\tau(x_\tau)$
\State $x_0 \sim V_0(x_0)$; \quad $\Delta \leftarrow 1/T$
\For{$i = 1$ to $T$}
    \State $x_{\tau+\Delta} \leftarrow x_\tau - \epsilon_\tau \nabla  V_\tau(x_\tau) \, d\tau + \sqrt{2\epsilon_\tau} \, dW_\tau$
    \State $\log w_{\tau+\Delta} \leftarrow \log w_\tau - \partial_\tau V_\tau(x_\tau) \, d\tau$
    \State $\tau \leftarrow \tau + \Delta$
    \If{$\text{ESS} < \text{ESS}_{\text{threshold}}$}
        \State $x_\tau \leftarrow \textsc{Resample}(x_\tau, w_\tau)$
        \State $w_\tau \leftarrow 0$
    \EndIf
\EndFor
\end{algorithmic}
\end{algorithm}

\paragraph{SCALLOP with SMC.} 
To extend \scalloptt to continuous-time SMC as SBG-SMC, we could simply replace $p^\theta$ with $p^\theta_1$. Noting that solving the above coupled system of SDE/ODE, one requires to calculate/estimate $p^\theta_1(x)$ for arbitrary $x$. To enable the estimation, one could follow \cite{ai2026f2d2} to use the reverse-mode likelihood estimation, described by \Cref{alg:reverse_mode_scallop}. Then the \scalloptt-SMC reads \Cref{alg:scallop_smc_sampling}.

\begin{algorithm}[H]
\caption{Reverse-mode likelihood estimation of \scalloptt}
\label{alg:reverse_mode_scallop}
\begin{algorithmic}[1] % [1] adds line numbers
\State \textbf{Input:} samples from model $x_1\sim p_1^\theta$, trained likelihood flow map $f_\theta=[u_\theta;D_\theta]$, reversed time schedule $\{t_i\}_{i=0}^N$ with $t_{i-1}>t_i$
\State \textbf{Output:} Estimated density of $x_1$, $p_N$

\State $p_0 \leftarrow 0$

\For{$i = 1$ \textbf{to} $N$}
    \State $(t, s) \leftarrow (t_{i-1}, t_i)$
    \State $x_i \leftarrow x_{i-1} - (s-t)u_\theta(x_{i-1}, t, s)$
    \State $\log p_i \leftarrow \log p_{i-1} - (s-t)D_\theta(x_{i-1}, t, s)$
\EndFor

\State $\log p_N\leftarrow \log p_N + \log p_0(x_0)$

\State \Return $p_N$
\end{algorithmic}
\end{algorithm}

\begin{algorithm}
\caption{\scalloptt-SMC Sampling}
\label{alg:scallop_smc_sampling}
\begin{algorithmic}[1]
\Require \# particles $K$, \# annealed distributions $T$, Energy annealing schedule $V_\tau(x_\tau)$
\State $x_0 \sim V_0(x_0)$; \quad $\Delta \leftarrow 1/T$
\For{$i = 1$ to $T$}
    \State $V_\tau(x_\tau)\leftarrow\text{\Cref{alg:reverse_mode_scallop}}$
    \State $x_{\tau+\Delta} \leftarrow x_\tau - \epsilon_\tau \nabla  V_\tau(x_\tau) \, d\tau + \sqrt{2\epsilon_\tau} \, dW_\tau$
    \State $\log w_{\tau+\Delta} \leftarrow \log w_\tau - \partial_\tau V_\tau(x_\tau) \, d\tau$
    \State $\tau \leftarrow \tau + \Delta$
    \If{$\text{ESS} < \text{ESS}_{\text{threshold}}$}
        \State $x_\tau \leftarrow \textsc{Resample}(x_\tau, w_\tau)$
        \State $w_\tau \leftarrow 0$
    \EndIf
\EndFor
\end{algorithmic}
\end{algorithm}

\subsection{Connecting SCALLOP and FALCON}
\label{app:sec:scallop-invertibility}
Estimating the log-density of a generated sample through (i) integrating the density-augmented PF-ODE (\scalloptt), or (ii) the reverse-mode \scalloptt, does not necessarily agree with each other. One could impose an additional loss. Recall that the likelihood flow map (\Cref{def:likelihood-flow-map}) is defined as
\begin{align}
    \Psi(x_t, t, s)=\begin{bmatrix}
        x_t\\0
    \end{bmatrix}+\int_t^s\begin{bmatrix}
         v_\tau(x_\tau)\\
        -\nabla\cdot v_\tau(x_\tau)
    \end{bmatrix}\dd\tau=\begin{bmatrix}
        x_s\\\log p_s(x_s)-\log p_t(x_t)
    \end{bmatrix}.
\end{align}
Feeding the generated $x_s$ for the reverse-mode calculation, we have
\begin{align}
    \Psi(x_s, s, t)=\begin{bmatrix}
        x_s\\0
    \end{bmatrix}+\int_s^t\begin{bmatrix}
         v_\tau(x_\tau)\\
        -\nabla\cdot v_\tau(x_\tau)
    \end{bmatrix}\dd\tau&=\begin{bmatrix}
        x_s+x_t-x_t-\int_t^sv_\tau(x_\tau)\dd\tau\\
        -\int_t^s -\nabla\cdot v_\tau(x_\tau)\dd\tau
    \end{bmatrix}\\
    &= \begin{bmatrix}
        x_s+x_t\\0
    \end{bmatrix}-\begin{bmatrix}
        x_t+\int_t^sv_\tau(x_\tau)\dd\tau\\
        \int_t^s -\nabla\cdot v_\tau(x_\tau)\dd\tau
    \end{bmatrix}\\
    &= \begin{bmatrix}
        x_s+x_t\\0
    \end{bmatrix}-\Psi(x_t, t, s).
\end{align}
Therefore, an additional constraint to enable reverse-mode likelihood flow map reads
\begin{align}
    \Psi(x_s, s, t)+\Psi(x_t, t, s)=\begin{bmatrix}
        x_s+x_t\\0
    \end{bmatrix}.
\end{align}
Recap that the likelihood flow map is parameterized as $\Psi_\theta(x, t, s)=\begin{bmatrix}
        x\\0
    \end{bmatrix}+(s-t)\begin{bmatrix}
        u_\theta(x, t, s)\\D_\theta(x, t, s)
    \end{bmatrix}$, the above constraint is therefore reduced to
\begin{align}
    \cancel{\begin{bmatrix}
        x_t\\0
    \end{bmatrix}}+(s-t)\begin{bmatrix}
        u_\theta(x_t, t, s)\\D_\theta(x_t, t, s)
    \end{bmatrix} +\cancel{\begin{bmatrix}
        x_s\\0
    \end{bmatrix}}+(t-s)\begin{bmatrix}
        u_\theta(x_s, s, t)\\D_\theta(x_s, s, t)
    \end{bmatrix}=\cancel{\begin{bmatrix}
        x_s+x_t\\0
    \end{bmatrix}},
\end{align}
which is equivalent to
\begin{align}
    u_\theta(x_t, t, s)=u_\theta(x_s, s, t)\quad\&\quad D_\theta(x_t, t, s)=D_\theta(x_s, s, t).
\end{align}
Noting that the constraint are imposed to a pair of $(x_t, x_s)$ that are generated through the velocity field $(v_t)_t$, which are not infeasible during training: (i) in a general case, $(v_t)_t$ is not available; and (ii) even though in the distillation case where $(v_t)_t$ is available from a pretrained model, it requires to integrate the ODE to get $x_s$ from $x_t$ or vice versa. For computational efficiency, one could use the likelihood flow map itself to form a self-constraint as follows:
\begin{align}
    \mathcal{L}_{\mathrm{SC}\text{-}v}(\theta;t, s) &= \left\|u_\theta(x_t, t, s)-u_\theta(u_\theta(x_t, t, s), s, t)\right\|^2\label{eq:self-constraint-reverse-v}\\
    \mathcal{L}_{\mathrm{SC}\text{-}D}(\theta;t, s) &= \left\|D_\theta(x_t, t, s)-D_\theta(D_\theta(x_t, t, s), s, t)\right\|^2\label{eq:self-constraint-reverse-D},
\end{align}
where \Cref{eq:self-constraint-reverse-v} coincides the invertibility loss proposed in FALCON and \Cref{eq:self-constraint-reverse-D} is the counterpart for log-density change.
