# Supplementary material for: Few-Step Boltzmann Generators via Scalable Likelihood Flow Maps
Source: arXiv:2606.29110 source file (2026-11-03)
Supplement: Supplementary file 2 [file new_error_bounds.tex]

\subsection{Error Quantification}\label{app:sec:error-bounds}

\subsubsection{Notation and Assumptions}\label{app:sec:error-bounds:notation}
We work on $\mathbb{R}^d$. Let $v_t^*$ denote the ground-truth velocity field
generating the probability path $(p_t)_{t\in[0,1]}$ through the continuity
equation $\partial_t p_t+\nabla\!\cdot(p_t v_t^*)=0$, and let $v_t$ denote the
velocity learned by the model, with marginal $p_t^v$ satisfying
$\partial_t p_t^v+\nabla\!\cdot(p_t^v v_t)=0$. Define the velocity error
\begin{align}
    \delta_t(x):=v_t(x)-v_t^*(x).
\end{align}
We adopt the parameterization $x_t=\alpha_t x_1+\gamma_t z$, $z\sim\mathcal{N}(0,I)$,
with $\gamma_t>0$ for $t\in[0,1)$ and $\gamma_1=0$.
We define the following quantities:
\begin{align}
    e_t^2:=\mathbb{E}_{p_t}\!\bigl[\|\delta_t(x_t)\|^2\bigr],\qquad
    B_t:=\|\delta_t\|_{L^\infty(\mathbb{R}^d)},\qquad
    S_t^2:=\mathbb{E}_{p_t}\!\bigl[\|\mathcal{D}\delta_t(x_t)\|^2\bigr],
\end{align}
where
\begin{align}
    \mathcal{D}f := \Delta f+\nabla\log p_t\cdot\nabla f
    \;=\;p_t^{-1}\nabla\!\cdot\!\bigl(p_t\,\nabla f\bigr)\label{eq:langevin-generator}
\end{align}
is the generator of the overdamped Langevin diffusion with invariant measure
$p_t$, applied component-wise to vector fields. We assume the following assumptions hold:
\begin{assumption}\label{ass:subgauss}
    $p_1$ is sub-Gaussian and $p_0=\mathcal{N}(0,I)$; hence every marginal
    $p_t$ is sub-Gaussian.
\end{assumption}
\begin{assumption}\label{ass:bounded}
    $B_t<\infty$ for $t\in[0,1]$.
\end{assumption}
\begin{assumption}\label{ass:hess}
    $S_t<\infty$ for $t\in[0,1]$, and integration by parts against $p_t$
    produces no boundary terms (e.g.\ $\delta_t$ has at most polynomial
    growth, which is implied by~\Cref{ass:bounded}).
\end{assumption}
\begin{assumption}\label{ass:bounded-4-moment}
    The 4th-order score moment of $p_1$ is strictly finite:
    \begin{align}
        J_4(p_1):=\mathbb{E}_{p_1}[\|\nabla\log p_1(x_1)\|^4]<\infty.
    \end{align}
\end{assumption}

We further define the following score factor for notational convenience:
\begin{align}
    G_t
    &:=
    \min\biggl(
        \frac{\sqrt{d(d+2)}}{\gamma_t^2},
        \frac{\sqrt{J_4(p_1)}}{\alpha_t^2}
    \biggr),
    \label{eq:score-factor-G}
\end{align}
with the extended-value convention that any term with zero denominator is
interpreted as $+\infty$. In particular, 
$G_t<\infty$, $G_0=\sqrt{d(d+2)}$, and
$G_1=\sqrt{J_4(p_1)}$.

\paragraph{Outline of the proof.}
The following error analysis proceeds from local to global: 
\begin{itemize}[leftmargin=*]
    \item First, we quantify the pointwise error introduced by replacing the intractable total derivative $\dd_t\log p_t^v$ with the surrogate $\widetilde{\dd_t\log p_t^v}$. This error decomposes into the score-velocity mismatch and the model-flow mismatched, which can be controlled using the velocity error $e_t$, the uniform error $B_t$, the score factor $G_t$ and the regularity of the generator $S_t$.
    \item Second, we propagate the pointwise error along the learned flow. Noting the surrogate likelihood is obtained by integrating the local estimator along the generation trajectories, we can control the likelihood estimation error $\Phi_t$ using the time integral of the pointwise mean square error up to the density-ratio constant $M_s^*$.

    \item Third, we use the likelihood estimation error to bound the error for importance sampling. Specifically, we show that the error of $\tilde H_t$ can be controlled by $\Phi_t$ as well as the second moment of the test function $h$, the density-ratio constants $M_t$ and $M_s^*$ and the factor $\kappa_t$.
    
    \item Finally, we use the similar logic to derive the resulting error of the learned estimator, accounting for finite-sample training error.

\end{itemize}

\subsubsection{Pointwise Error}

Along trajectories of the learned ODE $\dd x_t=v_t(x_t)\dd t$, the
instantaneous change-of-variables formula gives
\begin{align}
    \dd_t\log p_t^v(x_t)
    =\partial_t\log p_t^v(x_t)+\nabla\log p_t^v(x_t)\cdot v_t(x_t)
    =-\nabla\!\cdot v_t(x_t).
\end{align}
Because both $\nabla\log p_t^v$ and $\partial_t\log p_t^v$ are intractable, we replace them by $\nabla\log p_t$ and $\partial_t\log p_t$ respectively to obtain the estimator
\begin{align}
    \widetilde{\dd_t\log p_t^v}(x_t)
    :=\partial_t\log p_t(x_t)+\nabla\log p_t(x_t)\cdot v_t(x_t),
    \label{eq:dlogpv-dt-estimator}
\end{align}
where both $\nabla\log p_t$ and $\partial_t\log p_t$ could be estimated by a posterior expectation over the dataset \citep{song2021scorebasedgenerativemodelingstochastic,yu2025density}.

We further introduce the total derivative of the data density along the
ground-truth velocity field:
\begin{align}
    \dd_t\log p_t^{v^*}(x_t)
    &:=
    \partial_t\log p_t(x_t)+\nabla\log p_t(x_t)\cdot v_t^*(x_t)\\
    &=
    -\nabla\!\cdot v_t^*(x_t),
    \label{eq:dlogpvstar-dt}
\end{align}
where the last equality follows from the continuity equation
$\partial_t\log p_t+\nabla\log p_t\cdot v_t^*=-\nabla\!\cdot v_t^*$.

Define the pointwise error of the estimator as
\begin{align}
    \mathcal{E}_t(x_t)
    &:=
    \widetilde{\dd_t\log p_t^v}(x_t)-\dd_t\log p_t^v(x_t).
\end{align}
Adding and subtracting $\dd_t\log p_t^{v^*}(x_t)$, we can decompose the error as
\begin{align}
    \mathcal{E}_t(x_t)
    &=
    \underbrace{
    \widetilde{\dd_t\log p_t^v}(x_t)
    -
    \dd_t\log p_t^{v^*}(x_t)
    }_{\text{score--velocity mismatch}}
    +
    \underbrace{
    \dd_t\log p_t^{v^*}(x_t)
    -
    \dd_t\log p_t^v(x_t)
    }_{\text{model-flow mismatch}}.
    \label{eq:Et-decomposition}
\end{align}
The first term is given by
\begin{align}
    \widetilde{\dd_t\log p_t^v}(x_t)
    -
    \dd_t\log p_t^{v^*}(x_t)
    &=
    \partial_t\log p_t(x_t)+\nabla\log p_t(x_t)\cdot v_t(x_t) \notag\\
    &\quad -
    \partial_t\log p_t(x_t)-\nabla\log p_t(x_t)\cdot v_t^*(x_t)\\
    &=
    \nabla\log p_t(x_t)\cdot\delta_t(x_t).
\end{align}
The second term is given by
\begin{align}
    \dd_t\log p_t^{v^*}(x_t)
    -
    \dd_t\log p_t^v(x_t)
    &=
    -\nabla\!\cdot v_t^*(x_t)-\bigl(-\nabla\!\cdot v_t(x_t)\bigr)\\
    &=
    \nabla\!\cdot\delta_t(x_t).
\end{align}
Therefore,
\begin{align}
    \mathcal{E}_t(x_t)
    =
    \nabla\log p_t(x_t)\cdot\delta_t(x_t)
    +
    \nabla\!\cdot\delta_t(x_t).
\end{align}
Applying the triangle inequality to \Cref{eq:Et-decomposition}, followed by
$(a+b)^2\le 2a^2+2b^2$, gives
\begin{align}
    \mathcal{E}_t(x_t)^2
    &\leq
    2\left|
    \widetilde{\dd_t\log p_t^v}(x_t)
    -
    \dd_t\log p_t^{v^*}(x_t)
    \right|^2
    +
    2\left|
    \dd_t\log p_t^{v^*}(x_t)
    -
    \dd_t\log p_t^v(x_t)
    \right|^2\\
    &=
    2\bigl|\nabla\log p_t(x_t)\cdot\delta_t(x_t)\bigr|^2
    +
    2\bigl|\nabla\!\cdot\delta_t(x_t)\bigr|^2.
    \label{eq:Et-pointwise}
\end{align}

\begin{lemma}[Divergence error bound]\label{lem:div-bound}
    Under \Cref{ass:subgauss,ass:bounded,ass:hess}, for $t\in(0,1]$,
    \begin{align}
        \mathbb{E}_{p_t}\!\bigl[(\nabla\!\cdot\delta_t(x_t))^2\bigr]
        \;\le\;d\,e_t S_t.
    \end{align}
\end{lemma}

\begin{proof}
We proceed in three steps: reduce the squared divergence to the Frobenius
norm of the Jacobian, apply integration by parts to express that norm via
the Langevin generator~(\Cref{eq:langevin-generator}), then apply Cauchy--Schwarz in $L^2(p_t)$.

\paragraph{Step 1: Trace to Frobenius.}
Since
$\nabla\!\cdot\delta_t=\operatorname{tr}(\nabla\delta_t)
=\sum_{i=1}^d(\nabla\delta_t)_{ii}$,
applying Cauchy--Schwarz in the form $(\sum_{i=1}^d a_i)^2\le d\sum_{i=1}^d a_i^2$
to the diagonal entries and then adding back the (nonnegative) off-diagonal
entries gives
\begin{align}
    (\nabla\!\cdot\delta_t)^2
    \;\le\;d\sum_{i=1}^d(\nabla\delta_t)_{ii}^2
    \;\le\;d\sum_{i,j=1}^d(\nabla\delta_t)_{ij}^2
    \;=\;d\,\|\nabla\delta_t\|_F^2,
\end{align}
hence
$\mathbb{E}_{p_t}\!\bigl[(\nabla\!\cdot\delta_t(x_t))^2\bigr]
\le d\,\mathbb{E}_{p_t}\!\bigl[\|\nabla\delta_t(x_t)\|_F^2\bigr]$.

\paragraph{Step 2: Integration by parts.}
Decomposing row-wise,
$\|\nabla\delta_t\|_F^2=\sum_{j=1}^d\|\nabla\delta_t^j\|^2$, where
$\delta_t^j$ denotes the $j$-th component of $\delta_t$. For each $j$,
integration by parts against $p_t$ yields
\begin{align}
    \mathbb{E}_{p_t}\!\bigl[\|\nabla\delta_t^j(x_t)\|^2\bigr]
    &=\int \nabla\delta_t^j(x)\cdot\bigl(p_t(x)\,\nabla\delta_t^j(x)\bigr)\dd x \\
    &=-\int \delta_t^j(x)\,\nabla\!\cdot\!\bigl(p_t(x)\,\nabla\delta_t^j(x)\bigr)\dd x \\
    &=-\mathbb{E}_{p_t}\!\bigl[\delta_t^j(x_t)\,\mathcal{D}\delta_t^j(x_t)\bigr],
\end{align}
where the second equality uses the divergence theorem and the last
equality uses $\nabla\!\cdot(p_t\nabla f)=p_t\,\mathcal{D}f$ from the
definition of the Langevin generator~(\Cref{eq:langevin-generator}). The boundary contribution from
the divergence theorem,
\begin{equation}
    \lim_{R\to\infty}\int_{\partial B_R}\delta_t^j(x)\,p_t(x)\,
(\nabla\delta_t^j(x)\cdot\hat n)\dd S(x),
\end{equation}
vanishes because
$|\delta_t^j|\le B_t$ (\Cref{ass:bounded}), $p_t$ has sub-Gaussian tails
(\Cref{ass:subgauss}), and $\nabla\delta_t^j$ has at most polynomial
growth (\Cref{ass:hess}); the Gaussian decay of $p_t$ dominates the
surface area $\omega_{d-1}R^{d-1}$ and any polynomial growth of
$\nabla\delta_t^j$. Summing over $j$ gives the vector identity
\begin{align}
    \mathbb{E}_{p_t}\!\bigl[\|\nabla\delta_t(x_t)\|_F^2\bigr]
    =-\mathbb{E}_{p_t}\!\bigl[\delta_t(x_t)\cdot\mathcal{D}\delta_t(x_t)\bigr].
    \label{eq:frob-generator-identity}
\end{align}

\paragraph{Step 3: Cauchy--Schwarz in $L^2(p_t)$.}
By Cauchy--Schwarz,
\begin{align}
    \bigl|\mathbb{E}_{p_t}\!\bigl[\delta_t(x_t)\cdot\mathcal{D}\delta_t(x_t)\bigr]\bigr|
    \;\le\;\sqrt{\mathbb{E}_{p_t}\!\|\delta_t(x_t)\|^2}\,
           \sqrt{\mathbb{E}_{p_t}\!\|\mathcal{D}\delta_t(x_t)\|^2}
    \;=\;e_t S_t.
\end{align}
Combining the three steps yields the claim.
\end{proof}

\begin{lemma}[Mean-square error of the estimator]\label{lem:Et-bound}
    Under \Cref{ass:subgauss,ass:bounded,ass:hess,ass:bounded-4-moment}, for $t\in(0,1]$,
    \begin{align}
        \mathbb{E}_{p_t}\!\bigl[\mathcal{E}_t(x_t)^2\bigr]
        \;\le\;2\,e_t\!\left(d\,S_t+B_t \,G_t\right).
    \end{align}
\end{lemma}

\begin{proof}
By the triangle-inequality decomposition in \Cref{eq:Et-pointwise}, the
mean-square error splits into two terms:
\begin{align}
    \mathbb{E}_{p_t}\!\bigl[\mathcal{E}_t(x_t)^2\bigr]
    &\leq
    2\mathbb{E}_{p_t}\!\left[
    \left|
    \widetilde{\dd_t\log p_t^v}(x_t)
    -
    \dd_t\log p_t^{v^*}(x_t)
    \right|^2
    \right] \notag\\
    &\quad+
    2\mathbb{E}_{p_t}\!\left[
    \left|
    \dd_t\log p_t^{v^*}(x_t)
    -
    \dd_t\log p_t^v(x_t)
    \right|^2
    \right]\\
    &=
    2\mathbb{E}_{p_t}\!\left[
    \bigl|
    \nabla\log p_t(x_t)\cdot\delta_t(x_t)
    \bigr|^2
    \right]
    +
    2\mathbb{E}_{p_t}\!\left[
    \bigl|
    \nabla\!\cdot\delta_t(x_t)
    \bigr|^2
    \right].
\end{align}
We bound these two terms separately.

\paragraph{Model-flow mismatch.}
By \Cref{lem:div-bound},
\begin{align}
    \mathbb{E}_{p_t}\!\left[
    \left|
    \dd_t\log p_t^{v^*}(x_t)
    -
    \dd_t\log p_t^v(x_t)
    \right|^2
    \right]
    &=
    \mathbb{E}_{p_t}\!\left[
    \bigl|
    \nabla\!\cdot\delta_t(x_t)
    \bigr|^2
    \right]\\
    &\leq d\,e_tS_t.
\end{align}

\paragraph{Score--velocity mismatch.}
Pointwise Cauchy--Schwarz followed by Cauchy--Schwarz in $L^2(p_t)$ gives
\begin{align}
    \mathbb{E}_{p_t}\!\left[
    \left|
    \widetilde{\dd_t\log p_t^v}(x_t)
    -
    \dd_t\log p_t^{v^*}(x_t)
    \right|^2
    \right]
    &=
    \mathbb{E}_{p_t}\!\left[
    \bigl|
    \nabla\log p_t(x_t)\cdot\delta_t(x_t)
    \bigr|^2
    \right]\\
    &\le
    \sqrt{\mathbb{E}_{p_t}\!\|\nabla\log p_t(x_t)\|^4}\,
    \sqrt{\mathbb{E}_{p_t}\!\|\delta_t(x_t)\|^4}.
\end{align}
By Tweedie's formula, $\nabla\log p_t(x_t)=-\gamma_t^{-1}\,\mathbb{E}[z\mid x_t]$.
Applying conditional Jensen twice
($\|\mathbb{E}[z\mid x_t]\|^2\le\mathbb{E}[\|z\|^2\mid x_t]$ and then
$(\mathbb{E}[\|z\|^2\mid x_t])^2\le\mathbb{E}[\|z\|^4\mid x_t]$),
\begin{align}
    \mathbb{E}_{p_t}\!\|\nabla\log p_t(x_t)\|^4
    =\frac{1}{\gamma_t^4}\mathbb{E}_{p_t}\!\|\mathbb{E}[z\mid x_t]\|^4
    \le\frac{1}{\gamma_t^4}\mathbb{E}\|z\|^4=\frac{d(d+2)}{\gamma_t^4}.
\end{align}
By the Target Score Identity \citep{debortoli2024targetscorematching}, $\nabla\log p_t(x_t)=\alpha_t^{-1}\mathbb{E}[\nabla\log p_1(x_1)|x_t]$. Applying Jensen's inequality with \Cref{ass:bounded-4-moment},
\begin{align}
    \mathbb{E}_{p_t}\|\nabla\log p_t(x_t)\|^4
    =
    \frac{1}{\alpha_t^4}
    \mathbb{E}_{p_t}\|\mathbb{E}[\nabla\log p_1(x_1)|x_t]\|^4
    \leq
    \frac{1}{\alpha_t^4}
    \mathbb{E}\|\nabla\log p_1(x_1)\|^4
    =
    \frac{1}{\alpha_t^4}J_4(p_1).
\end{align}
Combining both bounds and taking square roots, we have
\begin{align}
    \sqrt{\mathbb{E}_{p_t}\!\|\nabla\log p_t(x_t)\|^4}
    \leq
    \min\biggl(
    \frac{\sqrt{d(d+2)}}{\gamma_t^2},
    \frac{\sqrt{J_4(p_1)}}{\alpha_t^2}
    \biggr)
    =
    G_t.
\end{align}
By \Cref{ass:bounded},
\begin{align}
    \mathbb{E}_{p_t}\!\|\delta_t(x_t)\|^4
    \leq
    B_t^2\mathbb{E}_{p_t}\!\|\delta_t(x_t)\|^2
    =
    B_t^2 e_t^2,
\end{align}
so $\sqrt{\mathbb{E}_{p_t}\!\|\delta_t(x_t)\|^4}\le B_t e_t$. Hence
\begin{align}
    \mathbb{E}_{p_t}\!\left[
    \left|
    \widetilde{\dd_t\log p_t^v}(x_t)
    -
    \dd_t\log p_t^{v^*}(x_t)
    \right|^2
    \right]
    \leq
    B_t e_t\,G_t.
\end{align}
Substituting both bounds into the decomposition gives
\begin{align}
    \mathbb{E}_{p_t}\!\bigl[\mathcal{E}_t(x_t)^2\bigr]
    \leq
    2e_t\left(dS_t+B_tG_t\right).
\end{align}
\end{proof}

\subsubsection{Error of Likelihood Estimation}
Recall the estimator $\widetilde{\dd_t\log p_t^v}$ from
\Cref{eq:dlogpv-dt-estimator}. We turn it into a surrogate log-density by
integrating it along the learned trajectory $\phi$ (where $x_t=\phi_t(x_0)$,
$x_0\sim p_0$), matching the exact log-density at the same initial condition:
\begin{align}
    \log\tilde p_t^v\bigl(\phi_t(x_0)\bigr)
    &:=\log p_0(x_0)+\int_0^t\!\widetilde{\dd_s\log p_s^v}\bigl(\phi_s(x_0)\bigr)\,ds,\\
    \log p_t^v\bigl(\phi_t(x_0)\bigr)
    &=\log p_0(x_0)+\int_0^t\!\dd_s\log p_s^v\bigl(\phi_s(x_0)\bigr)\,ds .
\end{align}
We define the likelihood-estimation error
$\Phi_t(x_t):=\log\tilde p_t^v(x_t)-\log p_t^v(x_t)$. Since the two
representations share the initial condition, $\Phi_0\equiv0$ and, subtracting,
\begin{align}
    \Phi_t\bigl(\phi_t(x_0)\bigr)
    =
    \int_0^t
    \Bigl(
    \widetilde{\dd_s\log p_s^v}
    -
    \dd_s\log p_s^v
    \Bigr)
    \bigl(\phi_s(x_0)\bigr)\,ds
    =
    \int_0^t \mathcal{E}_s\bigl(\phi_s(x_0)\bigr)\,ds .
    \label{eq:Phi-integral-rep}
\end{align}
This section bounds $\mathbb{E}_{p_t^v}[\Phi_t(x_t)^2]$; the next section
propagates it to the importance-sampling error.

\begin{proposition}[Likelihood-estimation error]\label{prop:phi-bound}
Under \Cref{ass:subgauss,ass:bounded,ass:hess,ass:bounded-4-moment} and quantities defined in \Cref{app:sec:error-bounds:notation}, suppose the
density-ratio constant $M_s^*:=\|p_s^v/p_s\|_{L^\infty}$ is finite for
$s\in[0,t]$ ($M_s^*=1$ when $v=v^*$). Then for every $t\in[0,1]$,
\begin{align}
    \mathbb{E}_{p_t^v}\!\bigl[\Phi_t(x_t)^2\bigr]
    \;\le\; t\int_0^t\! M_s^*\,\mathbb{E}_{p_s}\!\bigl[\mathcal{E}_s(x_s)^2\bigr]\,ds
    \;\le\; 2t\int_0^t\! M_s^*\,e_s\bigl(d\,S_s+B_s\,G_s\bigr)\,ds.
\end{align}
\end{proposition}

\begin{proof}
Because $x_t=\phi_t(x_0)$ pushes $p_0$ forward to $p_t^v$, the change of
variables and the integral representation \Cref{eq:Phi-integral-rep} give
\begin{align}
    \mathbb{E}_{p_t^v}\!\bigl[\Phi_t(x_t)^2\bigr]
    =
    \mathbb{E}_{p_0}\!\left[
    \left(
    \int_0^t\mathcal{E}_s(\phi_s(x_0))\,ds
    \right)^{\!2}
    \right]
    \le
    t\int_0^t\!\mathbb{E}_{p_0}\!\bigl[\mathcal{E}_s(\phi_s(x_0))^2\bigr]\,ds
    =
    t\int_0^t\!\mathbb{E}_{p_s^v}\!\bigl[\mathcal{E}_s(x_s)^2\bigr]\,ds,
\end{align}
where the inequality is Cauchy--Schwarz in $s$ (Jensen on $[0,t]$) and the last
equality again uses the pushforward $\phi_s{}_\#p_0=p_s^v$. Transferring each
inner expectation from $p_s^v$ to $p_s$,
\begin{align}
    \mathbb{E}_{p_s^v}\!\bigl[\mathcal{E}_s(x_s)^2\bigr]
    =
    \int \frac{p_s^v}{p_s}\,\mathcal{E}_s^2\,p_s\,dx
    \le
    M_s^*\,\mathbb{E}_{p_s}\!\bigl[\mathcal{E}_s(x_s)^2\bigr],
\end{align}
which proves the first inequality. The second follows by inserting
\Cref{lem:Et-bound}, $\mathbb{E}_{p_s}[\mathcal{E}_s^2]\le 2e_s(d\,S_s+B_sG_s)$.
\end{proof}

\subsubsection{Error of Importance Sampling}
For a test function $h:\mathbb{R}^d\to\mathbb{R}^k$ we wish to estimate
\begin{align}
    H_t:=\mathbb{E}_{p_t}\!\bigl[h(x_t)\bigr]
    =
    \mathbb{E}_{p_t^v}\!\left[\frac{p_t(x_t)}{p_t^v(x_t)}\,h(x_t)\right]
\end{align}
using samples from the learned flow. Since $p_t^v$ is intractable, we replace it
by the surrogate $\tilde p_t^v$ of the previous section, giving the estimand
\begin{align}
    \tilde H_t:=\mathbb{E}_{p_t^v}\!\left[\frac{p_t(x_t)}{\tilde p_t^v(x_t)}\,h(x_t)\right].
\end{align}
With $\Phi_t=\log\tilde p_t^v-\log p_t^v$ as above, a change of variables gives
\begin{align}
    H_t-\tilde H_t
    =
    \int p_t(x_t)\,h(x_t)\!\left(1-\frac{p_t^v(x_t)}{\tilde p_t^v(x_t)}\right)\!dx_t
    =
    \mathbb{E}_{p_t}\!\bigl[h(x_t)\,\bigl(1-e^{-\Phi_t(x_t)}\bigr)\bigr],
\end{align}
so by Cauchy--Schwarz in $L^2(p_t)$,
\begin{align}
    \|H_t-\tilde H_t\|
    \le
    \sqrt{\mathbb{E}_{p_t}\!\|h(x_t)\|^2}\,
    \sqrt{\mathbb{E}_{p_t}\!\bigl[(1-e^{-\Phi_t(x_t)})^2\bigr]}.
    \label{eq:IS-CS-1}
\end{align}
The mean value theorem gives $1-e^{-u}=u\,e^{-\xi}$ for some $\xi$ between $0$ and
$u$, hence $|1-e^{-u}|\le|u|\,e^{\max(-u,0)}$. Squaring and writing
$\kappa_t:=\|e^{\max(-\Phi_t,\,0)}\|_{L^\infty(p_t)}$,
\begin{align}
    \mathbb{E}_{p_t}\!\bigl[(1-e^{-\Phi_t(x_t)})^2\bigr]
    \le
    \mathbb{E}_{p_t}\!\bigl[\Phi_t(x_t)^2\,e^{2\max(-\Phi_t(x_t),0)}\bigr]
    \le
    \kappa_t^2\,\mathbb{E}_{p_t}\!\bigl[\Phi_t(x_t)^2\bigr].
    \label{eq:IS-CS-2}
\end{align}
The integral representation \Cref{eq:Phi-integral-rep} controls $\Phi_t$ along
the learned flow, i.e.\ under $p_t^v$; we therefore transfer the remaining
expectation from $p_t$ to $p_t^v$ using $M_t:=\|p_t/p_t^v\|_{L^\infty}$
($M_t=1$ when $v=v^*$):
\begin{align}
    \mathbb{E}_{p_t}\!\bigl[\Phi_t(x_t)^2\bigr]
    \le M_t\,\mathbb{E}_{p_t^v}\!\bigl[\Phi_t(x_t)^2\bigr].
    \label{eq:phi-transfer}
\end{align}
Applying \Cref{prop:phi-bound} to the right-hand side and combining with
\Cref{eq:IS-CS-1,eq:IS-CS-2} yields the main result.

\begin{theorem}[Importance-sampling error]\label{thm:IS}
    Under \Cref{ass:subgauss,ass:bounded,ass:hess,ass:bounded-4-moment} and with
    $\kappa_t,M_t,M_s^*<\infty$, for every $t\in[0,1]$,
    \begin{align}
        \|H_t-\tilde H_t\|
        \;\le\;
        \sqrt{\mathbb{E}_{p_t}\!\|h(x_t)\|^2}\;\kappa_t\sqrt{M_t}\,
        \sqrt{2t\int_0^t\! M_s^*\,e_s\!\left(d\,S_s+B_s
        G_s\right)\,ds}.
    \end{align}
    For equilibrium sampling from $p_1$ ($t=1$),
    \begin{align}
        \|H_1-\tilde H_1\|
        \;\le\;
        \sqrt{\mathbb{E}_{p_1}\!\|h(x_1)\|^2}\;\kappa_1\sqrt{M_1}\,
        \sqrt{2\int_0^1\! M_s^*\,e_s\!\left(d\,S_s+B_sG_s\right)\,ds}.
    \end{align}
\end{theorem}

\begin{remark}
    The constants $\kappa_t,M_t,M_s^*$ all reduce to $1$ in the well-specified
    limit $v\to v^*$, where $e_s\equiv0$ and both bounds vanish. They isolate the
    deviation of the sampling measure $p_t^v$ from the target $p_t$:
    \Cref{prop:phi-bound} controls the \emph{accumulated} likelihood error along
    the flow via $M_s^*$, while the extra factor $M_t$ in \Cref{eq:phi-transfer}
    converts that path-level guarantee into a target-level one. The local fidelity
    of the estimator itself is carried by \Cref{lem:Et-bound}.
\end{remark}

\subsubsection{Finite-Sample Training Error}\label{app:sec:finite-sample-training-error}

In the previous sections, we quantify the mismatch caused by using an
imperfect velocity field $v_t$ in place of the ground-truth velocity $v_t^*$ in the population limit. Next, we also incorporate the finite-sample errors from the two training stages, using similar derivations as above.

Let $D_t^\theta$ denote the learned total-score estimator. We use the terminology that, during the pretraining stage, the velocity field $v_t$ is trained to match $v_t^*$, while during the training stage, $D_t^\theta$ is trained to match $\widetilde{\dd_t\log p_t^v}$. We define the training-stage error
\begin{align}
    \varepsilon_{D,t}^2
    :=
    \mathbb{E}_{p_t^v}\!\left[
    \left|
    D_t^\theta(x_t)
    -
    \widetilde{\dd_t\log p_t^v}(x_t)
    \right|^2
    \right].
    \label{eq:D-training-error}
\end{align}
The final estimator is $D_t^\theta$ instead of $\widetilde{\dd_t\log p_t^v}$. As such, we define the final pointwise error as
\begin{align}
    \mathcal E_t^\theta(x_t)
    :=
    D_t^\theta(x_t)-\dd_t\log p_t^v(x_t).
\end{align}
Adding and subtracting $\widetilde{\dd_t\log p_t^v}(x_t)$, we have
\begin{align}
    \mathcal E_t^\theta(x_t)
    &=
    \underbrace{
    D_t^\theta(x_t)
    -
    \widetilde{\dd_t\log p_t^v}(x_t)
    }_{\text{training-stage error}}
    +
    \underbrace{
    \widetilde{\dd_t\log p_t^v}(x_t)
    -
    \dd_t\log p_t^v(x_t)
    }_{\text{pretraining velocity mismatch}}.
    \label{eq:theta-error-decomposition}
\end{align}
We further apply $(a+b)^2\leq 2a^2+2b^2$:
\begin{align}
    \mathbb{E}_{p_t^v}\!\left[
    \bigl(\mathcal E_t^\theta(x_t)\bigr)^2
    \right]
    &\leq
    2\mathbb{E}_{p_t^v}\!\left[
    \left|
    D_t^\theta(x_t)
    -
    \widetilde{\dd_t\log p_t^v}(x_t)
    \right|^2
    \right] \notag\\
    &\quad+
    2\mathbb{E}_{p_t^v}\!\left[
    \left|
    \widetilde{\dd_t\log p_t^v}(x_t)
    -
    \dd_t\log p_t^v(x_t)
    \right|^2
    \right].
    \label{eq:theta-error-split}
\end{align}
Observe that first term is exactly $\varepsilon_{D,t}^2$. For the second term, we use the density-ratio constant
\begin{align}
    M_t^*:=\left\|\frac{p_t^v}{p_t}\right\|_{L^\infty},
\end{align}
and apply \Cref{lem:Et-bound}. As such,
\begin{align}
    \mathbb{E}_{p_t^v}\!\left[
    \left|
    \widetilde{\dd_t\log p_t^v}(x_t)
    -
    \dd_t\log p_t^v(x_t)
    \right|^2
    \right]
    &=
    \int
    \frac{p_t^v(x)}{p_t(x)}
    \left|
    \widetilde{\dd_t\log p_t^v}(x)
    -
    \dd_t\log p_t^v(x)
    \right|^2
    p_t(x)\dd x\\
    &\leq
    M_t^*
    \mathbb{E}_{p_t}\!\left[
    \left|
    \widetilde{\dd_t\log p_t^v}(x_t)
    -
    \dd_t\log p_t^v(x_t)
    \right|^2
    \right]\\
    &\leq
    2M_t^*e_t\left(dS_t+B_tG_t\right).
\end{align}
Substituting the resulting bound into \Cref{eq:theta-error-split} gives
\begin{align}
    \mathbb{E}_{p_t^v}\!\left[
    \bigl(\mathcal E_t^\theta(x_t)\bigr)^2
    \right]
    \leq
    2\varepsilon_{D,t}^2
    +
    4M_t^*e_t\left(dS_t+B_tG_t\right).
    \label{eq:theta-local-error-bound}
\end{align}

\begin{proposition}[Finite-sample likelihood-estimation error]
\label{prop:finite-sample-likelihood-error}
Recall that $x_t=\phi_t(x_0)$ denotes the learned trajectory generated by $\dd x_t=v_t(x_t)\dd t$, where $x_0\sim p_0$. We define the surrogate likelihood induced by the learned total-score estimator $D_t^\theta$
\begin{align}
    \log \tilde p_t^{v,\theta}\bigl(\phi_t(x_0)\bigr)
    &:=
    \log p_0(x_0)
    +
    \int_0^t D_s^\theta\bigl(\phi_s(x_0)\bigr)\dd s.
\end{align}
Denote
\begin{align}
    \Phi_t^\theta(x_t)
    :=
    \log \tilde p_t^{v,\theta}(x_t)
    -
    \log p_t^v(x_t).
\end{align}
Under the assumptions of \Cref{lem:Et-bound}, and assuming
$M_s^*=\|p_s^v/p_s\|_{L^\infty}<\infty$ for $s\in[0,t]$, we have
\begin{align}
    \mathbb{E}_{p_t^v}\!\left[
    \bigl(\Phi_t^\theta(x_t)\bigr)^2
    \right]
    \leq
    t\int_0^t
    \left[
    2\varepsilon_{D,s}^2
    +
    4M_s^*e_s\left(dS_s+B_sG_s\right)
    \right]\dd s.
    \label{eq:finite-sample-likelihood-error}
\end{align}
\end{proposition}

\begin{proof}
Using the definitions of $\tilde p_t^{v,\theta}$ and $p_t^v$ along the learned trajectory,
\begin{align}
    \Phi_t^\theta\bigl(\phi_t(x_0)\bigr)
    =
    \int_0^t
    \left[
    D_s^\theta\bigl(\phi_s(x_0)\bigr)
    -
    \dd_s\log p_s^v\bigl(\phi_s(x_0)\bigr)
    \right]\dd s
    =
    \int_0^t
    \mathcal E_s^\theta\bigl(\phi_s(x_0)\bigr)\dd s.
\end{align}
Since $\phi_t{}_\#p_0=p_t^v$, using Cauchy--Schwarz in time
\begin{equation}
    \mathbb{E}_{p_t^v}\!\left[
    \bigl(\Phi_t^\theta(x_t)\bigr)^2
    \right]
    =
    \mathbb{E}_{p_0}\!\left[
    \left(
    \int_0^t
    \mathcal E_s^\theta\bigl(\phi_s(x_0)\bigr)\dd s
    \right)^2
    \right]\\
    \leq
    t\int_0^t
    \mathbb{E}_{p_0}\!\left[
    \bigl(
    \mathcal E_s^\theta\bigl(\phi_s(x_0)\bigr)
    \bigr)^2
    \right]\dd s\\
    =
    t\int_0^t
    \mathbb{E}_{p_s^v}\!\left[
    \bigl(
    \mathcal E_s^\theta(x_s)
    \bigr)^2
    \right]\dd s.
\end{equation}
One can apply \Cref{eq:theta-local-error-bound} at each time $s$ to obtain \Cref{eq:finite-sample-likelihood-error}.
\end{proof}

\begin{theorem}[Finite-sample importance-sampling error]
\label{thm:finite-sample-IS}
For a test function $h:\mathbb{R}^d\to\mathbb{R}^k$, define
\begin{align}
    H_t
    &:=
    \mathbb{E}_{p_t}[h(x_t)]
    =
    \mathbb{E}_{p_t^v}
    \left[
    \frac{p_t(x_t)}{p_t^v(x_t)}h(x_t)
    \right],
\end{align}
and the finite-sample estimand
\begin{align}
    \tilde H_t^\theta
    :=
    \mathbb{E}_{p_t^v}
    \left[
    \frac{p_t(x_t)}{\tilde p_t^{v,\theta}(x_t)}h(x_t)
    \right].
\end{align}
Further define
\begin{align}
    \kappa_t^\theta
    :=
    \left\|
    e^{\max(-\Phi_t^\theta,0)}
    \right\|_{L^\infty(p_t)},
    \qquad
    M_t
    :=
    \left\|
    \frac{p_t}{p_t^v}
    \right\|_{L^\infty}.
\end{align}
Then, under the assumptions of \Cref{prop:finite-sample-likelihood-error}, with
$\kappa_t^\theta,M_t<\infty$, we have
\begin{equation}
    \|H_t-\tilde H_t^\theta\|
    \leq
    \sqrt{\mathbb{E}_{p_t}\|h(x_t)\|^2}\;
    \kappa_t^\theta\sqrt{M_t} \notag\\
    \times
    \sqrt{
    t\int_0^t
    \left[
    2\varepsilon_{D,s}^2
    +
    4M_s^*e_s\left(dS_s+B_sG_s\right)
    \right]\dd s
    }.
    \label{eq:finite-sample-IS-error}
\end{equation}
For equilibrium sampling from $p_1$, we have
\begin{equation}
    \|H_1-\tilde H_1^\theta\|
    \leq
    \sqrt{\mathbb{E}_{p_1}\|h(x_1)\|^2}\;
    \kappa_1^\theta\sqrt{M_1} \notag\\
    \times
    \sqrt{
    \int_0^1
    \left[
    2\varepsilon_{D,s}^2
    +
    4M_s^*e_s\left(dS_s+B_sG_s\right)
    \right]\dd s
    }.
\end{equation}
\end{theorem}

\begin{proof}
We have
\begin{equation}
    H_t-\tilde H_t^\theta
    =
    \int p_t(x_t)h(x_t)
    \left(
    1-\frac{p_t^v(x_t)}{\tilde p_t^{v,\theta}(x_t)}
    \right)\dd x_t\\
    =
    \mathbb{E}_{p_t}\!\left[
    h(x_t)
    \left(
    1-e^{-\Phi_t^\theta(x_t)}
    \right)
    \right].
\end{equation}
Therefore, by Cauchy--Schwarz,
\begin{equation}
    \|H_t-\tilde H_t^\theta\|
    \leq
    \sqrt{\mathbb{E}_{p_t}\|h(x_t)\|^2}\,
    \sqrt{
    \mathbb{E}_{p_t}
    \left[
    \left(
    1-e^{-\Phi_t^\theta(x_t)}
    \right)^2
    \right]
    }.
\end{equation}
Using $|1-e^{-u}|\leq |u|e^{\max(-u,0)}$, we get
\begin{equation}
    \mathbb{E}_{p_t}
    \left[
    \left(
    1-e^{-\Phi_t^\theta(x_t)}
    \right)^2
    \right]
    \leq
    \mathbb{E}_{p_t}
    \left[
    \bigl(\Phi_t^\theta(x_t)\bigr)^2
    e^{2\max(-\Phi_t^\theta(x_t),0)}
    \right]\\
    \leq
    \bigl(\kappa_t^\theta\bigr)^2
    \mathbb{E}_{p_t}
    \left[
    \bigl(\Phi_t^\theta(x_t)\bigr)^2
    \right].
\end{equation}
Transferring the expectation from $p_t$ to $p_t^v$, we have
\begin{align}
    \mathbb{E}_{p_t}
    \left[
    \bigl(\Phi_t^\theta(x_t)\bigr)^2
    \right]
    \leq
    M_t
    \mathbb{E}_{p_t^v}
    \left[
    \bigl(\Phi_t^\theta(x_t)\bigr)^2
    \right].
\end{align}
Applying \Cref{prop:finite-sample-likelihood-error} completes the proof.
\end{proof}

We next discuss how the bound relate to sample sizes.

\begin{assumption}[Finite-sample learning rates]
\label{ass:finite-sample-rates}
Denote the number of samples used to train the velocity field $v_t$ as $n_v$,
and denote the number of samples used to train the total-score estimator $D_t^\theta$ as $n_D$. Assume that uniformly over $s\in[0,t]$,
\begin{align}
    \varepsilon_{D,s}(n_D)
    &\leq C_D n_D^{-\beta_D},\\
    e_{s,n_v}
    &\leq C_v n_v^{-\beta_v},\\
    B_{s,n_v}
    &\leq C_B,\\
    S_{s,n_v}
    &\leq C_S,
\end{align}
where $C_D,C_v,C_B,C_S>0,\beta_D,\beta_v>0$ are constants. Further assume that $G_s$ and $M_s^*$ are uniformly bounded
on $[0,t]$, i.e.
\begin{align}
    G_s\leq C_G,
    \qquad
    M_s^*\leq C_M,
    \qquad
    s\in[0,t].
\end{align}
\end{assumption}

\begin{corollary}[Sample-size dependence]
\label{cor:sample-size-dependence}
Under \Cref{ass:finite-sample-rates}, the local deployed-estimator error
satisfies
\begin{align}
    \mathbb{E}_{p_s^v}
    \left[
    \bigl(\mathcal E_s^\theta(x_s)\bigr)^2
    \right]
    =
    O(n_D^{-2\beta_D})
    +
    O(n_v^{-\beta_v}),
\end{align}
uniformly over $s\in[0,t]$. Consequently, the likelihood-estimation error follows that
\begin{align}
    \mathbb{E}_{p_t^v}
    \left[
    \bigl(\Phi_t^\theta(x_t)\bigr)^2
    \right]
    =
    O(t^2 n_D^{-2\beta_D})
    +
    O(t^2 n_v^{-\beta_v}),
\end{align}
and the resulting importance-sampling error satisfies
\begin{align}
    \|H_t-\tilde H_t^\theta\|
    =
    O(t n_D^{-\beta_D})
    +
    O(t n_v^{-\beta_v/2}).
\end{align}
In particular, if both stages achieve root-sample rates,
$\beta_D=\beta_v=1/2$, then
\begin{align}
    \|H_t-\tilde H_t^\theta\|
    =
    O(t n_D^{-1/2})
    +
    O(t n_v^{-1/4}).
\end{align}
Under the scenario that $t=1$, this becomes
\begin{align}
    \|H_1-\tilde H_1^\theta\|
    =
    O(n_D^{-1/2})
    +
    O(n_v^{-1/4}).
\end{align}
\end{corollary}

\begin{proof}
From \Cref{eq:theta-local-error-bound},
\begin{align}
    \mathbb{E}_{p_s^v}
    \left[
    \bigl(\mathcal E_s^\theta(x_s)\bigr)^2
    \right]
    &\leq
    2\varepsilon_{D,s}^2(n_D)
    +
    4M_s^*e_{s,n_v}
    \left(
    dS_{s,n_v}
    +
    B_{s,n_v}G_s
    \right).
\end{align}
By \Cref{ass:finite-sample-rates},
\begin{align}
    2\varepsilon_{D,s}^2(n_D)
    \leq
    2C_D^2n_D^{-2\beta_D},
\end{align}
and
\begin{align}
    4M_s^*e_{s,n_v}
    \left(
    dS_{s,n_v}
    +
    B_{s,n_v}G_s
    \right)
    \leq
    4C_M C_v
    \left(
    dC_S+C_BC_G
    \right)
    n_v^{-\beta_v}.
\end{align}
Therefore,
\begin{align}
    \mathbb{E}_{p_s^v}
    \left[
    \bigl(\mathcal E_s^\theta(x_s)\bigr)^2
    \right]
    =
    O(n_D^{-2\beta_D})
    +
    O(n_v^{-\beta_v}).
\end{align}
Substituting this bound into \Cref{prop:finite-sample-likelihood-error} gives
\begin{align}
    \mathbb{E}_{p_t^v}
    \left[
    \bigl(\Phi_t^\theta(x_t)\bigr)^2
    \right]
    &\leq
    t\int_0^t
    \left[
    O(n_D^{-2\beta_D})
    +
    O(n_v^{-\beta_v})
    \right]\dd s\\
    &=
    O(t^2 n_D^{-2\beta_D})
    +
    O(t^2 n_v^{-\beta_v}).
\end{align}
Finally, applying \Cref{thm:finite-sample-IS} and taking the square root yields
\begin{align}
    \|H_t-\tilde H_t^\theta\|
    =
    O(t n_D^{-\beta_D})
    +
    O(t n_v^{-\beta_v/2}).
\end{align}
The parametric-rate statement follows by setting
$\beta_D=\beta_v=1/2$.
\end{proof}
