# Supplementary material for: Few-Step Boltzmann Generators via Scalable Likelihood Flow Maps
Source: arXiv:2606.29110 source file (2026-11-03)
Supplement: Supplementary file 3 [file additional_experiments.tex]

\section{Additional Experiments}
