# Supplementary material for: Few-Step Boltzmann Generators via Scalable Likelihood Flow Maps
Source: arXiv:2606.29110 source file (2026-11-03)
Supplement: Supplementary file 4 [file error_bounds.tex]

% % \subsection{Error Quantification}\label{app:sec:error-bounds}
% % In this section, we discuss what and where the mismatch is, in the proposed estimators \Cref{eq:cond-total-derivative-estimator-restate,eq:cond-trace-estimator-restate} and their variants. To start, we first clarity two important and distinguihsed concepts--the \emph{model densities} $(p_t^v)_t$ and the \emph{data densities} $(p_t)_t$--where
% % \begin{itemize}
% %     \item $(p_t^v)_t$ are induced from the velocity $v_t$; while
% %     \item $(p_t)_t$ are induced either from the optimal velocity $v_t^*$ or the SIs (\Cref{eq:stochastic-interpolants-def}).
% % \end{itemize}
% % Before stepping into the details, we state our conclusion first:
% % \begin{theorem}
% %     For any $v_t$, integrating the estimator 
% %     \begin{align}
% %         \dd_t\log p_t^v(x_t)
% %         &\approx \partial_t\log p_t(x_t)+\nabla\log p_t(x_t)\cdot v_t(x_t)
% %         % :=\widetilde{\dd_t\log p_t^v(x_t)}
% %         \label{eq:cond-total-derivative-estimator-restate-for-mismatch},
% %     \end{align}
% %     along the dynamics $\dd x_t=v_t(x_t)\dd t$, yields unbiased estimators for $\bigl(p_t(x_t)\bigr)_t$. In particular, the estimations are unbiased for $\bigl(p_t^v(x_t)\bigr)_t$ if and only if $v_t\equiv v_t^*$ for all $t\in[0,1]$.
% % \end{theorem}

% % \begin{proof}

% % Directly apply the fundamental theorem of calculus.

% % \end{proof}

% % \paragraph{Error quantification with imperfect velocity.}
% % Given \textbf{any} velocity field $(v_t)_t$, the induced log model likelihood, $\log p_t^v$, preserves the aforementioned total-derivative formula:
% % \begin{align}
% %     \dd_t\log p_t^v(x_t) &= \partial_t\log p_t^v(x_t)+\nabla\log p_t^v(x_t)\cdot v_t(x_t).
% % \end{align}
% % While \Cref{eq:cond-total-derivative-estimator-restate-for-mismatch} estimates the $\dd_t\log p_t^v$ term by replacing the model scores, $\partial_t\log p_t^v$ and $\nabla\log p_t^v$, with the true scores, $\partial_t\log p_t$ and $\nabla\log p_t$, therefore raises mismatch on the \textbf{model likelihood estimation}.

% % % To quantify the mismatch, we suppose following assumptions are fulfilled:

% % % \begin{assumption}
% % % The error bound between $v_t$ and $v_t^*$ are given by
% % % \begin{align}\label{assump:bound-on-velocity}
% % %     \mathbb{E}_{p_t}[\|v_t(x_t)-v_t^*(x_t)\|^2]\leq \mathcal{E}^v_t.
% % % \end{align}
% % % \end{assumption}
% % % \begin{assumption}\label{assump:uniform-bound-on-score}
% % %     The score, $\nabla\log p_t$, are bounded almost everywhere
% % %     \begin{align}
% % %         C_t=\sup_{x\in\mathrm{supp}(p_t)}\|\nabla\log p_t(x)\|^2_\infty<\infty.
% % %     \end{align}
% % % \end{assumption}

% % % % \tony{The second assumption on the score is very strong, we should somehow alleviate it...}

% % % Let us recap the conditional total derivative estimator:
% % % \begin{align}
% % %     \dd_t\log p_t(x_t)&= -\mathbb{E}\biggl[\frac{z}{\gamma_t}\cdot\Bigl(v_t(x_t)-\tilde v_t(x_t|x_0,x_1)\Bigr)+\frac{\dot\gamma_t}{\gamma_t}d\Big|x_t\biggr],
% % % \end{align}
% % % where the true estimator is unbiased iff $v_t=v_t^*$, i.e.
% % % \begin{align}
% % %     \dd_t\log p_t^{v^*}(x_t)&= -\mathbb{E}\biggl[\frac{z}{\gamma_t}\cdot\Bigl(v_t^*(x_t)-\tilde v_t(x_t|x_0,x_1)\Bigr)+\frac{\dot\gamma_t}{\gamma_t}d\Big|x_t\biggr].
% % % \end{align}
% % % Hence, the error bound at time $t$ is given by:
% % % \begin{align}
% % %     \mathbb{E}_{p_t}\|\dd_t\log p_t(x_t)-\dd_t\log p_t^{v^*}(x_t)\|^2,
% % % \end{align}
% % % where
% % % \begin{align}
% % %     &\|\dd_t\log p_t(x_t)-\dd_t\log p_t^{v^*}(x_t)\|^2 \\
% % %     =& \biggl\| \mathbb{E}\biggl[\frac{z}{\gamma_t}\cdot\Bigl(v_t(x_t)-\tilde v_t(x_t|x_0,x_1)\Bigr)-\frac{Z}{\gamma_t}\cdot\Bigl(v_t^*(x_t)-\tilde v_t(x_t|x_0,x_1)\Bigr)\Big|x_t\biggr]\biggr\|^2\\
% % %     =& \biggl\| \mathbb{E}\biggl[\frac{Z}{\gamma_t}\cdot\Bigl(v_t(x_t)-v^*_t(x_t)\Bigr)\Big|x_t\biggr]\biggr\|^2\\
% % %     =& \biggl\| \frac{1}{\gamma_t}\mathbb{E}\biggl[z\Big|x_t\biggr]\cdot\Bigl(v_t(x_t)-v^*_t(x_t)\Bigr)\biggr\|^2\\
% % %     =& \biggl\| \nabla\log p_t(x_t)\cdot\Bigl(v_t(x_t)-v^*_t(x_t)\Bigr)\biggr\|^2.
% % % \end{align}
% % % Hence,
% % % \begin{align}
% % %     \mathbb{E}_{p_t}\|\dd_t\log p_t(x_t)-\dd_t\log p_t^{v^*}(x_t)\|^2 &= \mathbb{E}_{p_t}\biggl[\Big\| \nabla\log p_t(x_t)\cdot\Bigl(v_t(x_t)-v^*_t(x_t)\Bigr)\Bigr\|^2\biggr]\\
% % %     &\leq\mathbb{E}_{p_t}\biggl[\Big\| \nabla\log p_t(x_t)\Bigr\|^2_\infty\Big\|v_t(x_t)-v^*_t(x_t)\Bigr\|^2\biggr]\\
% % %     &\overset{(i)}{\leq}\mathbb{E}_{p_t}\biggl[C_t\Big\|v_t(x_t)-v^*_t(x_t)\Bigr\|^2\biggr]
% % % \end{align}
% % % where $(i)$ is by \Cref{assump:uniform-bound-on-score}. And hence
% % % \begin{align}
% % %     \int \mathbb{E}_{p_t}\|\dd_t\log p_t(x_t)-\dd_t\log p_t^{v^*}(x_t)\|^2\dd t&\leq\int C_t \mathbb{E}_{p_t}\biggl[C_t\Big\|v_t(x_t)-v^*_t(x_t)\Bigr\|^2\biggr]\dd t\overset{(ii)}{\leq}\int C_t\mathcal{E}_t^v\dd t,
% % % \end{align}
% % % where $(ii)$ is by \Cref{assump:bound-on-velocity}.

% % % \hanlin{Alternative based on fourth order moment}

% % To quantify the mismatch, we suppose following assumptions are fulfilled:

% % \begin{assumption}\label{assump:bound-on-velocity-L4}
% %     The fourth moment of the velocity error is bounded:
% %     \begin{align}
% %         \mathbb{E}_{p_t}\left[\left\|v_t(x_t)-v_t^*(x_t)\right\|^4\right]\leq \mathcal{E}^{v, (4)}_t.
% %     \end{align}
% % \end{assumption}

% % \begin{assumption}\label{assump:moment-bound-on-score}
% %     The score function $\nabla\log p_t$ has a bounded fourth moment:
% %     \begin{align}
% %         M_t = \mathbb{E}_{p_t}[\|\nabla\log p_t(x_t)\|^4] < \infty.
% %     \end{align}
% % \end{assumption}

% % Let us recap the conditional total derivative estimator:
% % \begin{align}
% %     \dd_t\log p_t(x_t)&= -\mathbb{E}\biggl[\frac{z}{\gamma_t}\cdot\Bigl(v_t(x_t)-\tilde v_t(x_t|x_0,x_1)\Bigr)+\frac{\dot\gamma_t}{\gamma_t}d\Big|x_t\biggr],
% % \end{align}
% % where the true estimator is unbiased iff $v_t=v_t^*$, i.e.
% % \begin{align}
% %     \dd_t\log p_t^{v^*}(x_t)&= -\mathbb{E}\biggl[\frac{z}{\gamma_t}\cdot\Bigl(v_t^*(x_t)-\tilde v_t(x_t|x_0,x_1)\Bigr)+\frac{\dot\gamma_t}{\gamma_t}d\Big|x_t\biggr].
% % \end{align}
% % Hence, the error bound at time $t$ is given by:
% % \begin{align}
% %     \mathbb{E}_{p_t}\|\dd_t\log p_t(x_t)-\dd_t\log p_t^{v^*}(x_t)\|^2,
% % \end{align}
% % where
% % \begin{align}
% %     &\|\dd_t\log p_t(x_t)-\dd_t\log p_t^{v^*}(x_t)\|^2 \\
% %     =& \biggl\| \mathbb{E}\biggl[\frac{z}{\gamma_t}\cdot\Bigl(v_t(x_t)-\tilde v_t(x_t|x_0,x_1)\Bigr)-\frac{z}{\gamma_t}\cdot\Bigl(v_t^*(x_t)-\tilde v_t(x_t|x_0,x_1)\Bigr)\Big|x_t\biggr]\biggr\|^2\\
% %     =& \biggl\| \mathbb{E}\biggl[\frac{z}{\gamma_t}\cdot\Bigl(v_t(x_t)-v^*_t(x_t)\Bigr)\Big|x_t\biggr]\biggr\|^2\\
% %     =& \biggl\| \frac{1}{\gamma_t}\mathbb{E}\biggl[z\Big|x_t\biggr]\cdot\Bigl(v_t(x_t)-v^*_t(x_t)\Bigr)\biggr\|^2\\
% %     =& \biggl\| \nabla\log p_t(x_t)\cdot\Bigl(v_t(x_t)-v^*_t(x_t)\Bigr)\biggr\|^2.
% % \end{align}
% % Hence,
% % \begin{align}
% %     \mathbb{E}_{p_t}\|\dd_t\log p_t(x_t)-\dd_t\log p_t^{v^*}(x_t)\|^2 
% %     &= \mathbb{E}_{p_t}\biggl[\Big| \nabla\log p_t(x_t)\cdot\Bigl(v_t(x_t)-v^*_t(x_t)\Bigr)\Big|^2\biggr]\\
% %     &\overset{(i)}{\leq}\mathbb{E}_{p_t}\biggl[\Big\| \nabla\log p_t(x_t)\Bigr\|^2\Big\|v_t(x_t)-v^*_t(x_t)\Bigr\|^2\biggr]\\
% %     &\overset{(ii)}{\leq} \sqrt{\mathbb{E}_{p_t}\biggl[\Big\| \nabla\log p_t(x_t)\Bigr\|^4\biggr]} \sqrt{\mathbb{E}_{p_t}\biggl[\Big\|v_t(x_t)-v^*_t(x_t)\Bigr\|^4\biggr]}\\
% %     &\overset{(iii)}{\leq} \sqrt{M_t \mathcal{E}^{v, (4)}_t},
% % \end{align}
% % where $(i)$ follows from the Cauchy-Schwarz inequality for vectors, $(ii)$ is due to the Cauchy-Schwarz inequality for expectations (Hölder's inequality), and $(iii)$ is by \Cref{assump:bound-on-velocity-L4} and \Cref{assump:moment-bound-on-score}. 

% % Therefore,
% % \begin{align}
% %     \mathbb{E}_{p_t}\|\dd_t\log p_t(x_t)-\dd_t\log p_t^{v^*}(x_t)\|^2 \leq \sqrt{M_t \mathcal{E}^{v, (4)}_t}.
% % \end{align}

% % \subsubsection{Another one}
% % The true estimator for the likelihood should be 
% % \begin{align}
% %     \dd_t\log p_t^v(x_t)
% %     &= \partial_t\log p_t^v(x_t)+\nabla\log p_t^v(x_t)\cdot v_t(x_t)=-\nabla\cdot v_t(x_t),
% % \end{align}
% % While the one we use is
% % \begin{align}
% %     \dd_t\log p_t^v(x_t)
% %     &\approx \partial_t\log p_t(x_t)+\nabla\log p_t(x_t)\cdot v_t(x_t):=\widetilde{\dd_t\log p_t^v(x_t)}.\label{eq:dlogpv-dt-estimator}
% % \end{align}
% % Since
% % \begin{align}
% %     -\nabla\cdot v_t^*(x_t)=\partial_t\log p_t(x_t)+\nabla\log p_t(x_t)\cdot v_t^*(x_t),
% % \end{align}
% % we are effectively using the following approximation
% % \begin{align}
% %     \widetilde{\dd_t\log p_t^v(x_t)}
% %     &= -\nabla\cdot v_t^*(x_t)-\nabla\log p_t(x_t)\cdot v_t^*(x_t)+\nabla\log p_t(x_t)\cdot v_t(x_t)\\
% %     &= -\nabla\cdot v_t^*(x_t)+\nabla\log p_t(x_t)\cdot \bigl(v_t(x_t)-v_t^*(x_t)\bigr).
% % \end{align}
% % And hence, if given access to $\partial_t\log p_t$ and $\nabla\log p_t$, the pointwise error of the above approximation is given by
% % \begin{align}
% %     &\|\widetilde{\dd_t\log p_t^v(x_t)}-{\dd_t\log p_t^v(x_t)}\|^2\\
% %     =&\Bigl\|-\nabla\cdot v_t^*(x_t)+\nabla\log p_t(x_t)\cdot \bigl(v_t(x_t)-v_t^*(x_t)\bigr)+\nabla\cdot v_t(x_t)\Bigr\|^2\\
% %     =&\Bigl\|\nabla\cdot \bigl(v_t(x_t)-v_t^*(x_t)\bigr)+\nabla\log p_t(x_t)\cdot \bigl(v_t(x_t)-v_t^*(x_t)\bigr)\Bigr\|^2\\
% %     \leq& 2\Bigl\|\nabla\cdot \bigl(v_t(x_t)-v_t^*(x_t)\bigr)\Bigr\|^2+2\Bigl\|\nabla\log p_t(x_t)\cdot \bigl(v_t(x_t)-v_t^*(x_t)\bigr)\Bigr\|^2\\
% %     \leq& 2\Bigl\|\nabla\cdot \bigl(v_t(x_t)-v_t^*(x_t)\bigr)\Bigr\|^2+2\Bigl\|\nabla\log p_t(x_t)\Bigr\|^2_\infty\Bigl\| v_t(x_t)-v_t^*(x_t)\Bigr\|^2,
% % \end{align}
% % where the obstacles are in two ways: (1) the divergence difference $\Bigl\|\nabla\cdot \bigl(v_t(x_t)-v_t^*(x_t)\bigr)\Bigr\|^2$, which should impose some assumptions on both the learned $v_t$ and the true $v_t^*$; and (2) the bound on the score, $\Bigl\|\nabla\log p_t(x_t)\Bigr\|^2_\infty$, where an uniform bound is very strong.

% % \hanlin{
% % We take expectation over $p_t$.

% % To quantify the mismatch, we suppose following assumptions are fulfilled:

% % \begin{assumption}\label{assump:bound-on-velocity-L4}
% %     The fourth moment of the velocity error is bounded:
% %     \begin{align}
% %         \mathbb{E}_{p_t}\left[\left\|v_t(x_t)-v_t^*(x_t)\right\|^4\right]\leq \mathcal{E}^{v, (4)}_t.
% %     \end{align}
% % \end{assumption}

% % \begin{assumption}\label{assump:moment-bound-on-score}
% %     The score function $\nabla\log p_t$ has a bounded fourth moment:
% %     \begin{align}
% %         M_t = \mathbb{E}_{p_t}[\|\nabla\log p_t(x_t)\|^4] < \infty.
% %     \end{align}
% % \end{assumption}

% % The bound involves two terms: $\E_{p_t}\Bigl\|\nabla\cdot \bigl(v_t(x_t)-v_t^*(x_t)\bigr)\Bigr\|^2$ and $\E_{p_t}\Bigl\|\nabla\log p_t(x_t)\cdot \bigl(v_t(x_t)-v_t^*(x_t)\bigr)\Bigr\|^2$. Next we look into these two terms independently.

% % For the first term, we have

% % For the second term, we have
% % \begin{align}
% %     \mathbb{E}_{p_t}\|\dd_t\log p_t(x_t)-\dd_t\log p_t^{v^*}(x_t)\|^2 
% %     &= \mathbb{E}_{p_t}\biggl[\Big| \nabla\log p_t(x_t)\cdot\Bigl(v_t(x_t)-v^*_t(x_t)\Bigr)\Big|^2\biggr]\\
% %     &\overset{(i)}{\leq}\mathbb{E}_{p_t}\biggl[\Big\| \nabla\log p_t(x_t)\Bigr\|^2\Big\|v_t(x_t)-v^*_t(x_t)\Bigr\|^2\biggr]\\
% %     &\overset{(ii)}{\leq} \sqrt{\mathbb{E}_{p_t}\biggl[\Big\| \nabla\log p_t(x_t)\Bigr\|^4\biggr]} \sqrt{\mathbb{E}_{p_t}\biggl[\Big\|v_t(x_t)-v^*_t(x_t)\Bigr\|^4\biggr]}\\
% %     &\overset{(iii)}{\leq} \sqrt{M_t \mathcal{E}^{v, (4)}_t},
% % \end{align}
% % where $(i)$ follows from the Cauchy-Schwarz inequality for vectors, $(ii)$ is due to the Cauchy-Schwarz inequality for expectations (Hölder's inequality), and $(iii)$ is by \Cref{assump:bound-on-velocity-L4} and \Cref{assump:moment-bound-on-score}. 
% % }

% % Once we fix the above bound, we could further include the error bound on learning by using the triangle inequality:
% % \begin{align}
% %     \|D^\theta_t(x_t)-\dd_t\log p_t^v(x_t)\|^2&=\|D_t^\theta(x_t)-\widetilde{\dd_t\log p_t^v(x_t)}+\widetilde{\dd_t\log p_t^v(x_t)}-{\dd_t\log p_t^v(x_t)}\|^2\\
% %     &\leq 2\|D_t^\theta(x_t)-\widetilde{\dd_t\log p_t^v(x_t)}\|^2+2\|\widetilde{\dd_t\log p_t^v(x_t)}-{\dd_t\log p_t^v(x_t)}\|^2
% % \end{align}

% % \subsection{What is the mismatch: the true estimated item with our estimator}
% % Thought the estimator \Cref{eq:cond-total-derivative-estimator-restate} results in biased estimation for the log model density, $\log p_t^v$, it actually returns into an unbiased estomition for the log \textbf{true density} $\log p_t$. Notice that for any $v_t$, the chain rule still reads
% % \begin{align}
% %     \dd_t\log p_t(x_t) &= \partial_t\log p_t(x_t)+\nabla\log p_t(x_t)\cdot v_t(x_t),
% % \end{align}
% % as long as $(x_t)_t$ follow the dynamics induced by $(v_t)_t$. That means, \Cref{eq:cond-total-derivative-estimator-restate} is actually:
% % \begin{itemize}
% %     \item an \textbf{unbiased} estimator for $\dd_t\log p_t(x_t)$;
% %     \item but an \textbf{biased} estimator for $\dd_t\log p_t^v(x_t)$,
% % \end{itemize}
% % where the bias can be understood as the mismatch between $\dd_t\log p_t^v$ and $\dd_t\log p_t$, and therefore mismatch between $\log p_t^v$ and $\log p_t$.

% % \paragraph{Correcting the bias for model density.} To debias the estimator for log model density, one should quantify the mismatch between $\log p_t$ and $\log p_t^v$, which turns out the be a density-ratio estimation problem. In principle, if we have an unbiased estimator for $\log p_t$, then we only need the density ratio to debias:
% % \begin{align}
% %     r_t^v(x)=\frac{p_t^v(x)}{p_t(x)} \Longrightarrow p_t^v(x)=r_t^v(x)p_t(x),
% % \end{align}
% % which can be estimated through training a classifier. In such a way, one could further tilt/guide the sampler to generate samples from another distribution $q$. In terms of the total derivative, the unbiased estimator for $\dd_t\log p_t^v$ can be written as:
% % \begin{align}
% %     \dd_t\log p_t^v(x_t)
% %     &= \dd_t\log p_t(x_t)+\dd_t\log r_t^v(x_t).    
% % \end{align}

% % % \begin{align}
% % %     \dd_t\log p_t^v(x_t)
% % %     &= \partial_t\log p_t^v(x_t)+\nabla\log p_t^v(x_t)\cdot v_t(x_t)\\
% % %     &= \partial_t\log p_t(x_t)+\nabla\log p_t(x_t)\cdot v_t(x_t) \notag\\
% % %     &\quad+ \partial_t\bigl(\log p_t^v(x_t)-\log p_t(x_t)\bigr)+\bigl(\nabla\log p_t^v(x_t)-\nabla\log p_t(x_t)\bigr)\cdot v_t(x_t).
% % % \end{align}
% % % Let
% % % \begin{align}
% % %     r_t^v(x)=\frac{p_t^v(x)}{p_t(x)},
% % % \end{align}
% % % the above estimator can be written as:
% % % \begin{align}
% % %     \dd_t\log p_t^v(x_t)
% % %     &=\partial_t\log p_t(x_t)+\nabla\log p_t(x_t)\cdot v_t(x_t) + \dd_t\log r_t^v(x_t),
% % % \end{align}
% % % where $r_t^v$ can be estimated by simply training a time-dependent classifier to distinguish $(x_t)_t$ and $(x_t^v)_t$ at each time step $t$.


% % \subsection{Could the mismatch be a bless?}
% % We introduce the bias of the proposed estimator, \Cref{eq:cond-total-derivative-estimator-restate}, for model density estimation, and a potential way to debias it, in the aforementioned sections. In this part, we focus on one question:

% % \begin{center}
% % \textit{Can we use the unbiased data density estimator in any applications?}
% % \end{center}

% % We provide a positive answer on the \emph{free energy difference estimation} problem, though whom is usually formalized as an importance sampling problem that requires the model density.

% % \paragraph{A brief introduction to free energy estimation.} Given a state $A$ with associated energy function $U_A$, which defines the Boltzmann/equilibrium distribution as $p_A(x)\propto\exp(-U_A(x))$, the \emph{free energy} of $A$ is defined as the negative log partition function
% % \begin{align}
% %     F_A=-\log Z_A=-\log \int\exp(-U_A(x))dx.
% % \end{align}
% % Given another state $B$ with energy function $U_B$, the free energy difference between $A$ and $B$ is conventionally defined as
% % \begin{align}
% %     \Delta F_{AB}=F_B-F_A=-\log\frac{\int\exp(-U_B(x))dx}{\int\exp(-U_A(x))dx}.
% % \end{align}
% % The free energy difference can be estimated using the importance sampling principle:
% % \begin{align}
% %     \Delta F_{AB}=-\log\mathbb{E}_A[\exp(U_A(X)-U_B(X))]=\log\mathbb{E}_B[\exp(U_B(X)-U_A(X))],
% % \end{align}
% % which is known as \emph{Free Energy Perturbation} (FEP).

% % \paragraph{Target FEP: free energy difference estimation via transport.} Let $T:\mathbb{R}^d\rightarrow\mathbb{R}^d$ a measurable bijection that transports samples from $p_A$ to $p_B$, i.e. $T_\# p_A=p_B$. Then,
% % \begin{align}
% %     \log p_B(x_B)-\log p_A(x_A)=-\log|\mathrm{det}(\mathcal{J}_{T}(x_A))|,\quad\text{where }x_B=T(x_A).
% % \end{align}
% % Therefore, the free energy difference can be expressed as
% % \begin{align}
% %     \Delta F_{AB}&=U_B(x_B)-U_A(x_A)-\log|\mathrm{det}(\mathcal{J}_{T}(x_A))|:=W_{AB}(x_A, x_B),\label{eq:generalized-work}
% % \end{align}
% % where $W_{AB}$ is also known as the \emph{generalized work}. Taking an expectation over $P_A$ and noting that $W$ is constant w.r.t. $x_A$ in this case, we have
% % \begin{align}
% %     \Delta F_{AB}=\mathbb{E}_{p_A}[W_{AB}(x_A, x_B)]=-\log\mathbb{E}_{p_A}[\exp(-W_{AB}(x_A, x_B))],
% % \end{align}
% % with $x_B=T(x_A)$,
% % which is known as the \emph{Jarzynski equality}. By symmetry,
% % \begin{align}
% %     \Delta F_{AB}=\log\mathbb{E}_{P_B}[\exp(W_{AB}(x_A,x_B))],\quad \text{with }x_A=T^{-1}(x_B).
% % \end{align}
% % Remarkably, the following properties hold:
% % \begin{enumerate}
% %     \item The Jarzynski equalities remain valid even when the transport map is imperfect (i.e. $T_\# p_A\neq p_B$). In such practical scenarios, we typically introduce two distinct, approximate mappings, $T_{A\rightarrow B}$ and $T_{B\rightarrow A}$, to model the forward and reverse transformations.
% %     \item When the transport map $T$ is perfect, the estimator of $\Delta F_{AB}$ has 0 variance, because the work remains constant for any $x_B=T(x_A)$.
% %     \item When the transport, $T$, is constructed via a continuous-time flow defined by a time-dependent velocity field $(v_t)_t$, mapping from $p_0=p_A$ to $p_1=p_B$, we have
% % \begin{align}
% %     -\log|\mathrm{det}(\mathcal{J}_{T}(x_A))|=-\int_0^1\nabla\cdot v_t(x_t)\dd t=\int_0^1{\dd_t\log p_t^v(x_t)}\dd t
% % \end{align} 
% % \end{enumerate}

% % \paragraph{Target FEP with our estimator.} According to \Cref{app:sec:error-bounds}, the conditional total derivative estimator, \Cref{eq:cond-total-derivative-estimator}, is an unbiased estimator for the total derivative $\dd_t\log p_t$ under the perfect velocity field $(v_t)_t$. Therefore, considering a mapping $T_{v^*}$ induced by $(v_t^*)_t$ and plugging the unbiased estimator into \Cref{eq:generalized-work}, we have an unbiased estimator for the work:
% % \begin{align}
% %     \widehat{W}_{AB}^v(x_A,x_B)=U_B(x_B)-U_A(x_A) + \int_0^1\widetilde{\dd_t\log p_t^v(x_t)}\dd t,
% % \end{align}
% % where $x_A:=x_0\sim p_A=p_0$ and $x_B:=x_1=x_A+\int_0^1v_t(x_t)\dd t$. Intuitively, the velocity field $(v_t)_t$ is providing a low-variance path for estimating the generalized work, and $v_t\equiv v_t^*$ for all $t$ achieves the minimum variance.

% % \subsection{New}
% % For notational convenience, we define {$v_t$ as the imperfect velocity as learned by the model, $v_t^*$ as the ground truth velocity induced by the probability path,} $\delta_t=v_t-v_t^*$, $e_t^2=\mathbb{E}_{p_t}[\|\delta_t(x_t)\|^2]$, $B_t=\|v_t-v_t^*\|_{L_\infty}$, $\mathcal{D}=\Delta+\nabla\log p_t\cdot\nabla$, and $S_t^2=\mathbb{E}_{p_t}[\|\mathcal{D}\delta_t(x)\|^2]$.
% % \begin{assumption}
% %     The target distribution $p_1$ is sub-Gaussian and $p_0=\mathcal{N}(0,I)$. Therefore, the marginals $(p_t)_t$ are sub-Gaussian as well.
% % \end{assumption}
% % \begin{assumption}
% %     $B_t=\|v_t-v_t^*\|_{L_\infty}<\infty$.
% % \end{assumption}
% % \begin{assumption}
% %     $S_t<\infty$, i.e. $v_t,v_t^*$ have bounded Hessians in $L^2(p_t)$.
% % \end{assumption}
% % The true estimator for the likelihood should be 
% % \begin{align}
% %     \dd_t\log p_t^v(x_t)
% %     &= \partial_t\log p_t^v(x_t)+\nabla\log p_t^v(x_t)\cdot v_t(x_t)=-\nabla\cdot v_t(x_t),
% % \end{align}
% % While the one we use is
% % \begin{align}
% %     \dd_t\log p_t^v(x_t)
% %     &\approx \partial_t\log p_t(x_t)+\nabla\log p_t(x_t)\cdot v_t(x_t):=\widetilde{\dd_t\log p_t^v(x_t)}.\label{eq:dlogpv-dt-estimator}
% % \end{align}
% % Since
% % \begin{align}
% %     -\nabla\cdot v_t^*(x_t)=\partial_t\log p_t(x_t)+\nabla\log p_t(x_t)\cdot v_t^*(x_t),
% % \end{align}
% % we are effectively using the following approximation
% % \begin{align}
% %     \widetilde{\dd_t\log p_t^v(x_t)}
% %     &= -\nabla\cdot v_t^*(x_t)-\nabla\log p_t(x_t)\cdot v_t^*(x_t)+\nabla\log p_t(x_t)\cdot v_t(x_t)\\
% %     &= -\nabla\cdot v_t^*(x_t)+\nabla\log p_t(x_t)\cdot \bigl(v_t(x_t)-v_t^*(x_t)\bigr).
% % \end{align}
% % \hanlin{Define $\mathcal{E}_t(x_t) = \widetilde{\dd_t\log p_t^v(x_t)}-{\dd_t\log p_t^v(x_t)}$ because we use it later for error of importance sampling}
% % And hence, if given access to $\partial_t\log p_t$ and $\nabla\log p_t$, the pointwise error of the above approximation is given by
% % \begin{align}
% %     \mathcal{E}_t(x_t)^{2}:=&\|\widetilde{\dd_t\log p_t^v(x_t)}-{\dd_t\log p_t^v(x_t)}\|^2\\
% %     =&\Bigl\|-\nabla\cdot v_t^*(x_t)+\nabla\log p_t(x_t)\cdot \bigl(v_t(x_t)-v_t^*(x_t)\bigr)+\nabla\cdot v_t(x_t)\Bigr\|^2\\
% %     =&\Bigl\|\nabla\cdot \bigl(v_t(x_t)-v_t^*(x_t)\bigr)+\nabla\log p_t(x_t)\cdot \bigl(v_t(x_t)-v_t^*(x_t)\bigr)\Bigr\|^2\\
% %     \leq& 2\Bigl\|\nabla\cdot \bigl(v_t(x_t)-v_t^*(x_t)\bigr)\Bigr\|^2+2\Bigl\|\nabla\log p_t(x_t)\cdot \bigl(v_t(x_t)-v_t^*(x_t)\bigr)\Bigr\|^2
% % \end{align}
% % Based on the Tweedie's formula:
% % \begin{align}
% %     \mathbb{E}_{p_t}\|\nabla\log p_t(x_t)\|^2=\mathbb{E}_{p_t}\|\frac{1}{\gamma_t}\mathbb{E}[z|x_t]\|^2\leq\frac{1}{\gamma_t^2}\mathbb{E}[\|z\|^2]=\frac{d}{\gamma_t^2},
% % \end{align}
% % and
% % \begin{align}
% %     \mathbb{E}_{p_t}\|\nabla\log p_t(x_t)\|^4=\mathbb{E}_{p_t}\|\frac{1}{\gamma_t}\mathbb{E}[z|x_t]\|^4\leq\frac{1}{\gamma_t^4}\mathbb{E}[\|z\|^4]=\frac{d(d+2)}{\gamma_t^4},
% % \end{align}
% % whenever $\gamma_t>0$.
% % The first term can be bounded by the Frobenius norm
% % \begin{align}
% %     \mathbb{E}_{p_t}\Bigl\|\nabla\cdot \bigl(v_t(x_t)-v_t^*(x_t)\bigr)\Bigr\|^2\leq d\mathbb{E}_{p_t}\Bigl\|\nabla\delta_t(x_t)\Bigr\|^2_F,
% % \end{align}
% % \hanlin{Applying integration by parts, and assuming the boundary terms vanish at infinity due to $p_t$ being sub-Gaussian,} it can be rewritten as follows under assumptions (1-3),
% % \begin{align}
% %     \mathbb{E}_{p_t}\Bigl\|\nabla\delta_t(x_t)\Bigr\|^2_F &= -\mathbb{E}_{p_t}[\delta_t(x_t)\cdot\mathcal{D}\delta_t(x_t)]\leq\sqrt{\mathbb{E}_{p_t}[\|\delta_t(x_t)\|^2]}\sqrt{\mathbb{E}_{p_t}[\|\mathcal{D}\delta_t(x_t)\|^2]}=e_tS_t
% % \end{align}
% %  The second term is bounded by
% % \begin{align}
% % \mathbb{E}_{p_t}\Bigl[\bigl(\nabla\log p_t(x_t)\cdot \delta_t(x_t)\bigr)^2\Bigr] &\leq \mathbb{E}_{p_t}\Bigl[\|\nabla\log p_t(x_t)\|^2 \|\delta_t(x_t)\|^2\Bigr] \\
% % &\leq \sqrt{\mathbb{E}_{p_t}\bigl[\|\nabla\log p_t(x_t)\|^4\bigr]} \sqrt{\mathbb{E}_{p_t}\bigl[\|\delta_t(x_t)\|^4\bigr]}\\
% % &\leq \frac{\sqrt{d(d+2)}}{\gamma_t^2}\sqrt{\mathbb{E}_{p_t}\bigl[\|\delta_t(x_t)\|^4\bigr]}\\
% % & \leq \frac{\sqrt{d(d+2)}}{\gamma_t^2}\sqrt{\mathbb{E}_{p_t}\bigl[B_t^2\|\delta_t(x_t)\|^2\bigr]}=\frac{\sqrt{d(d+2)}}{\gamma_t^2}B_te_t.
% % \end{align}
% % Overall,
% % \begin{align}
% %     \mathbb{E}_{p_t}|\widetilde{\dd_t\log p_t^v(x_t)}-{\dd_t\log p_t^v(x_t)}|^2\leq 2e_t\biggl(S_td+\frac{\sqrt{d(d+2)}}{\gamma_t^2}B_t\biggr).
% % \end{align}

% % \tony{This is not enough, overall, we want a bound on $\|\log p_t^v-\widetilde{\log p_t^v}\|$ and the below error bound regarding to IS.}

% % \paragraph{Error of Importance Sampling.} The propagated error occurs when applying the estimated likelihood for importance sampling. For any test function $h$, we care the expected quantity
% % \begin{align}
% %     H_t=\mathbb{E}_{p_t}[h(x_t)]=\mathbb{E}_{p_t^v}[\frac{p_t(x_t)}{p_t^v(x_t)}h(x_t)].
% % \end{align}
% % In particular, we are interested in the case of $t=1$ for equilibrium sampling. When using the proposed estimator, we approximate
% % \begin{align}
% %     H_t\approx\tilde H_t=\mathbb{E}_{p_t^v}[\frac{p_t(x_t)}{\tilde p_t^v(x_t)}h(x_t)].
% % \end{align}
% % We would  like to quantify
% % \begin{align}
% %     \|H_t-\tilde H_t\|&=\biggl\|\int p_t^v(x)h(x_t)\biggl(\frac{p_t(x_t)}{ p_t^v(x_t)}-\frac{p_t(x_t)}{\tilde p_t^v(x_t)}\biggr)\dd x_t\biggr\|= \biggl\|\int p_t(x_t)h(x_t)\biggl(1-\frac{p_t^v(x_t)}{\tilde p_t^v(x_t)}\biggr)\dd x_t\biggr\|.
% % \end{align}
% % Let $\Phi_t(x_t)=\log \tilde p_t^v(x_t)-\log p_t^v(x_t)=\int_0^t\mathcal{E}_s(x_s)\dd s$ and apply the Cauchy-Schwarz inequality, we have
% % \begin{align}
% %     \|H_t-\tilde H_t\|= \biggl\|\int p_t(x_t)h(x_t)\biggl(1-e^{-\Phi_t(x_t)}\biggr)\dd x_t\biggr\|\leq \sqrt{\mathbb{E}_{p_t}\| h(x_t)\|^2}\sqrt{\mathbb{E}_{p_t}| 1-e^{-\Phi_t(x_t)}|^2}.
% % \end{align}
% % By using $|1-e^{-u}|\leq |u|e^{\max(-u,0)}$, we could further upper bound
% % \begin{align}
% %     \|H_t-\tilde H_t\| \leq \sqrt{\mathbb{E}_{p_t}\| h(x_t)\|^2}\sqrt{\mathbb{E}_{p_t}[\Phi_t(x_t)^2e^{2\max(-\Phi_t(x_t), 0)}]}\leq \sqrt{\mathbb{E}_{p_t}\| h(x_t)\|^2}\kappa_t\sqrt{\mathbb{E}_{p_t}[\Phi_t(x_t)^2]},
% % \end{align}
% % where $\kappa_t=\|e^{\max(-\Phi_t(x_t), 0)}\|_{L^\infty}$. Then we would like to bound $\sqrt{\mathbb{E}_{p_t}[\Phi_t(x_t)^2]}$ through the bound on $\sqrt{\mathbb{E}_{p_t}[\mathcal{E}_t(x_t)^2]}$ derived above. Since $x_t$ is generated through push forwarding $x_0\sim p_0$ through a deterministic map defined by the PF-ODE, we have
% % \begin{align}
% %     {\mathbb{E}_{p_t}[\Phi_t(x_t)^2]}=\mathbb{E}_{p_0}\biggl[\biggl(\int_0^t\mathcal{E}_s(x_s)\dd s\biggr)^2\biggr]\leq t\int_0^t\mathbb{E}_{p_0}[\mathcal{E}_s(x_s)^2]\dd s=t\int_0^t\mathbb{E}_{p_s}[\mathcal{E}_s(x_s)^2]\dd s.
% % \end{align}
% % Combing all, we have
% % \begin{align}
% %     \|H_t-\tilde H_t\| \leq \sqrt{\mathbb{E}_{p_t}\| h(x_t)\|^2}\kappa_t\sqrt{2t\int_0^t e_s\biggl(S_sd+\frac{\sqrt{d(d+2)}}{\gamma_s^2}B_s\biggr)\dd s}
% % \end{align}


% \subsection{Error Quantification}\label{app:sec:error-bounds}

% \subsubsection{Notation and Assumptions}\label{app:sec:error-bounds:notation}
% We work on $\mathbb{R}^d$. Let $v_t^*$ denote the ground-truth velocity field
% generating the probability path $(p_t)_{t\in[0,1]}$ through the continuity
% equation $\partial_t p_t+\nabla\!\cdot(p_t v_t^*)=0$, and let $v_t$ denote the
% velocity learned by the model, with marginal $p_t^v$ satisfying
% $\partial_t p_t^v+\nabla\!\cdot(p_t^v v_t)=0$. Define the velocity error
% \begin{align}
%     \delta_t(x):=v_t(x)-v_t^*(x).
% \end{align}
% We adopt the parameterization $x_t=\alpha_t x_1+\gamma_t z$, $z\sim\mathcal{N}(0,I)$,
% with $\gamma_t>0$ for $t\in[0,1)$ and $\gamma_1=0$.
% We define the following quantities:
% \begin{align}
%     e_t^2:=\mathbb{E}_{p_t}\!\bigl[\|\delta_t(x_t)\|^2\bigr],\qquad
%     B_t:=\|\delta_t\|_{L^\infty(\mathbb{R}^d)},\qquad
%     S_t^2:=\mathbb{E}_{p_t}\!\bigl[\|\mathcal{D}\delta_t(x_t)\|^2\bigr],
% \end{align}
% where
% \begin{align}
%     \mathcal{D}f := \Delta f+\nabla\log p_t\cdot\nabla f
%     \;=\;p_t^{-1}\nabla\!\cdot\!\bigl(p_t\,\nabla f\bigr)\label{eq:langevin-generator}
% \end{align}
% is the generator of the overdamped Langevin diffusion with invariant measure
% $p_t$, applied component-wise to vector fields. We assume the following assumptions hold:
% \begin{assumption}\label{ass:subgauss}
%     $p_1$ is sub-Gaussian and $p_0=\mathcal{N}(0,I)$; hence every marginal
%     $p_t$ is sub-Gaussian.
% \end{assumption}
% \begin{assumption}\label{ass:bounded}
%     $B_t<\infty$ for $t\in[0,1]$.
% \end{assumption}
% \begin{assumption}\label{ass:hess}
%     $S_t<\infty$ for $t\in[0,1]$, and integration by parts against $p_t$
%     produces no boundary terms (e.g.\ $\delta_t$ has at most polynomial
%     growth, which is implied by~\Cref{ass:bounded}).
% \end{assumption}
% \begin{assumption}\label{ass:bounded-4-moment}
%     The 4th-order score moment of $p_1$ is strictly finite:
%     \begin{align}
%         J_4(p_1):=\mathbb{E}_{p_1}[\|\nabla\log p_1(x_1)\|^4]<\infty.
%     \end{align}
% \end{assumption}

% We further define the following score factor for notational convenience:
% \begin{align}
%     G_t
%     &:=
%     \min\biggl(
%         \frac{\sqrt{d(d+2)}}{\gamma_t^2},
%         \frac{\sqrt{J_4(p_1)}}{\alpha_t^2}
%     \biggr),
%     \label{eq:score-factor-G}
% \end{align}
% with the extended-value convention that any term with zero denominator is
% interpreted as $+\infty$. In particular, 
% $G_t<\infty$, $G_0=\sqrt{d(d+2)}$ and
% $G_1=\sqrt{J_4(p_1)}$.

% \subsubsection{Pointwise Error}

% Along trajectories of the learned ODE $\dd x_t=v_t(x_t)\dd t$, the
% instantaneous change-of-variables formula gives
% \begin{align}
%     \dd_t\log p_t^v(x_t)
%     =\partial_t\log p_t^v(x_t)+\nabla\log p_t^v(x_t)\cdot v_t(x_t)
%     =-\nabla\!\cdot v_t(x_t).
% \end{align}
% Because both $\nabla\log p_t^v$ and $\partial_t\log p_t^v$ are intractable, we replace them by $\nabla\log p_t$ and $\partial_t\log p_t$ respectively to obtain the estimator
% \begin{align}
%     \widetilde{\dd_t\log p_t^v}(x_t)
%     :=\partial_t\log p_t(x_t)+\nabla\log p_t(x_t)\cdot v_t(x_t),
%     \label{eq:dlogpv-dt-estimator}
% \end{align}
% where both $\nabla\log p_t$ and $\partial_t\log p_t$ could be estimated by a posterior expectation over the dataset \citep{song2021scorebasedgenerativemodelingstochastic,yu2025density}.
% Using the continuity equation
% $\partial_t\log p_t+\nabla\log p_t\cdot v_t^*=-\nabla\!\cdot v_t^*$ in
% \eqref{eq:dlogpv-dt-estimator},
% \begin{align}
%     \widetilde{\dd_t\log p_t^v}(x_t)
%     =-\nabla\!\cdot v_t^*(x_t)+\nabla\log p_t(x_t)\cdot\delta_t(x_t).
% \end{align}
% The pointwise error of the estimator is therefore
% \begin{align}
%     \mathcal{E}_t(x_t)
%     &:=\widetilde{\dd_t\log p_t^v}(x_t)-\dd_t\log p_t^v(x_t)\\
%     &=\nabla\!\cdot\delta_t(x_t)+\nabla\log p_t(x_t)\cdot\delta_t(x_t),
% \end{align}
% and by $(a+b)^2\le 2a^2+2b^2$,
% \begin{align}
%     \mathcal{E}_t(x_t)^2
%     \le 2\bigl|\nabla\!\cdot\delta_t(x_t)\bigr|^2
%        +2\bigl|\nabla\log p_t(x_t)\cdot\delta_t(x_t)\bigr|^2.
%     \label{eq:Et-pointwise}
% \end{align}

% \begin{lemma}[Divergence error bound]\label{lem:div-bound}
%     Under \Cref{ass:subgauss,ass:bounded,ass:hess}, for $t\in(0,1]$,
%     \begin{align}
%         \mathbb{E}_{p_t}\!\bigl[(\nabla\!\cdot\delta_t(x_t))^2\bigr]
%         \;\le\;d\,e_t S_t.
%     \end{align}
% \end{lemma}

% \begin{proof}
% We proceed in three steps: reduce the squared divergence to the Frobenius
% norm of the Jacobian, apply integration by parts to express that norm via
% the Langevin generator~(\Cref{eq:langevin-generator}), then apply Cauchy--Schwarz in $L^2(p_t)$.

% \paragraph{Step 1: Trace to Frobenius.}
% Since
% $\nabla\!\cdot\delta_t=\operatorname{tr}(\nabla\delta_t)
% =\sum_{i=1}^d(\nabla\delta_t)_{ii}$,
% applying Cauchy--Schwarz in the form $(\sum_{i=1}^d a_i)^2\le d\sum_{i=1}^d a_i^2$
% to the diagonal entries and then adding back the (nonnegative) off-diagonal
% entries gives
% \begin{align}
%     (\nabla\!\cdot\delta_t)^2
%     \;\le\;d\sum_{i=1}^d(\nabla\delta_t)_{ii}^2
%     \;\le\;d\sum_{i,j=1}^d(\nabla\delta_t)_{ij}^2
%     \;=\;d\,\|\nabla\delta_t\|_F^2,
% \end{align}
% hence
% $\mathbb{E}_{p_t}\!\bigl[(\nabla\!\cdot\delta_t(x_t))^2\bigr]
% \le d\,\mathbb{E}_{p_t}\!\bigl[\|\nabla\delta_t(x_t)\|_F^2\bigr]$.

% \paragraph{Step 2: Integration by parts.}
% Decomposing row-wise,
% $\|\nabla\delta_t\|_F^2=\sum_{j=1}^d\|\nabla\delta_t^j\|^2$, where
% $\delta_t^j$ denotes the $j$-th component of $\delta_t$. For each $j$,
% integration by parts against $p_t$ yields
% \begin{align}
%     \mathbb{E}_{p_t}\!\bigl[\|\nabla\delta_t^j(x_t)\|^2\bigr]
%     &=\int \nabla\delta_t^j(x)\cdot\bigl(p_t(x)\,\nabla\delta_t^j(x)\bigr)\dd x \\
%     &=-\int \delta_t^j(x)\,\nabla\!\cdot\!\bigl(p_t(x)\,\nabla\delta_t^j(x)\bigr)\dd x \\
%     &=-\mathbb{E}_{p_t}\!\bigl[\delta_t^j(x_t)\,\mathcal{D}\delta_t^j(x_t)\bigr],
% \end{align}
% where the second equality uses the divergence theorem and the last
% equality uses $\nabla\!\cdot(p_t\nabla f)=p_t\,\mathcal{D}f$ from the
% definition of the Langevin generator~(\Cref{eq:langevin-generator}). The boundary contribution from
% the divergence theorem,
% \begin{equation}
%     \lim_{R\to\infty}\int_{\partial B_R}\delta_t^j(x)\,p_t(x)\,
% (\nabla\delta_t^j(x)\cdot\hat n)\dd S(x),
% \end{equation}
% vanishes because
% $|\delta_t^j|\le B_t$ (\Cref{ass:bounded}), $p_t$ has sub-Gaussian tails
% (\Cref{ass:subgauss}), and $\nabla\delta_t^j$ has at most polynomial
% growth (\Cref{ass:hess}); the Gaussian decay of $p_t$ dominates the
% surface area $\omega_{d-1}R^{d-1}$ and any polynomial growth of
% $\nabla\delta_t^j$. Summing over $j$ gives the vector identity
% \begin{align}
%     \mathbb{E}_{p_t}\!\bigl[\|\nabla\delta_t(x_t)\|_F^2\bigr]
%     =-\mathbb{E}_{p_t}\!\bigl[\delta_t(x_t)\cdot\mathcal{D}\delta_t(x_t)\bigr].
%     \label{eq:frob-generator-identity}
% \end{align}

% \paragraph{Step 3: Cauchy--Schwarz in $L^2(p_t)$.}
% By Cauchy--Schwarz,
% \begin{align}
%     \bigl|\mathbb{E}_{p_t}\!\bigl[\delta_t(x_t)\cdot\mathcal{D}\delta_t(x_t)\bigr]\bigr|
%     \;\le\;\sqrt{\mathbb{E}_{p_t}\!\|\delta_t(x_t)\|^2}\,
%            \sqrt{\mathbb{E}_{p_t}\!\|\mathcal{D}\delta_t(x_t)\|^2}
%     \;=\;e_t S_t.
% \end{align}
% Combining the three steps yields the claim.
% \end{proof}

% \begin{lemma}[Mean-square error of the estimator]\label{lem:Et-bound}
%     Under \Cref{ass:subgauss,ass:bounded,ass:hess,ass:bounded-4-moment}, for $t\in(0,1]$,
%     \begin{align}
%         \mathbb{E}_{p_t}\!\bigl[\mathcal{E}_t(x_t)^2\bigr]
%         \;\le\;2\,e_t\!\left(d\,S_t+B_t \,G_t\right).
%     \end{align}
% \end{lemma}

% \begin{proof}
% We bound the two terms in \eqref{eq:Et-pointwise} separately.

% % \paragraph{First term.} We first relate the divergence to the Frobenius norm
% % of the Jacobian. Since
% % $\nabla\!\cdot\delta_t=\operatorname{tr}(\nabla\delta_t)=\sum_{i=1}^d(\nabla\delta_t)_{ii}$,
% % applying Cauchy--Schwarz in the form
% % $(\sum_{i=1}^d a_i)^2\le d\sum_{i=1}^d a_i^2$ to the diagonal entries and then
% % adding back the (nonnegative) off-diagonal entries gives
% % \begin{align}
% %     \bigl(\nabla\!\cdot\delta_t\bigr)^2
% %     \;\le\;d\sum_{i=1}^d(\nabla\delta_t)_{ii}^2
% %     \;\le\;d\sum_{i,j=1}^d(\nabla\delta_t)_{ij}^2
% %     \;=\;d\,\|\nabla\delta_t\|_F^2,
% % \end{align}
% % and hence
% % $\mathbb{E}_{p_t}[(\nabla\!\cdot\delta_t(x_t))^2]\le d\,\mathbb{E}_{p_t}[\|\nabla\delta_t(x_t)\|_F^2]$.

% % It remains to bound the Frobenius norm. Decomposing row-wise,
% % $\|\nabla\delta_t\|_F^2=\sum_{j=1}^d\|\nabla\delta_t^j\|^2$, where
% % $\delta_t^j$ denotes the $j$-th component of $\delta_t$. For each $j$,
% % integration by parts against $p_t$ yields
% % \begin{align}
% %     \mathbb{E}_{p_t}\!\bigl[\|\nabla\delta_t^j(x_t)\|^2\bigr]
% %     &=\int \nabla\delta_t^j(x)\cdot\bigl(p_t(x)\,\nabla\delta_t^j(x)\bigr)\dd x \\
% %     &=-\int \delta_t^j(x)\,\nabla\!\cdot\!\bigl(p_t(x)\,\nabla\delta_t^j(x)\bigr)\dd x \\
% %     &=-\mathbb{E}_{p_t}\!\bigl[\delta_t^j(x_t)\,\mathcal{D}\delta_t^j(x_t)\bigr],
% % \end{align}
% % where the second equality uses the divergence theorem and the last
% % equality uses $\nabla\!\cdot(p_t\nabla f)=p_t\,\mathcal{D}f$ from the
% % definition of the Langevin generator. The boundary term from the
% % divergence theorem is
% % \begin{align}
% %     \lim_{R\to\infty}\int_{\partial B_R} \delta_t^j(x)\,p_t(x)\,
% %     \bigl(\nabla\delta_t^j(x)\cdot\hat n\bigr)\dd S(x),
% % \end{align}
% % which vanishes because $|\delta_t^j|\le B_t$ (\Cref{ass:bounded}),
% % $p_t$ has sub-Gaussian tails (\Cref{ass:subgauss}), and $\nabla\delta_t^j$
% % grows at most polynomially (\Cref{ass:hess}); the Gaussian decay of $p_t$
% % dominates the surface area $\omega_{d-1}R^{d-1}$ and any polynomial
% % growth of $\nabla\delta_t^j$. Summing over $j$ recovers the vector
% % inner product:
% % \begin{align}
% %     \mathbb{E}_{p_t}\!\bigl[\|\nabla\delta_t(x_t)\|_F^2\bigr]
% %     =-\sum_{j=1}^d\mathbb{E}_{p_t}\!\bigl[\delta_t^j(x_t)\,\mathcal{D}\delta_t^j(x_t)\bigr]
% %     =-\mathbb{E}_{p_t}\!\bigl[\delta_t(x_t)\cdot\mathcal{D}\delta_t(x_t)\bigr].
% % \end{align}
% \paragraph{First term.} By \Cref{lem:div-bound},
% $\mathbb{E}_{p_t}\!\bigl[(\nabla\!\cdot\delta_t(x_t))^2\bigr]\le d\,e_t S_t$.

% \paragraph{Second term.} Pointwise Cauchy--Schwarz followed by
% Cauchy--Schwarz in $L^2(p_t)$ gives
% \begin{align}
%     \mathbb{E}_{p_t}\!\bigl[(\nabla\log p_t(x_t)\cdot\delta_t(x_t))^2\bigr]
%     \le\sqrt{\mathbb{E}_{p_t}\!\|\nabla\log p_t(x_t)\|^4}\,
%         \sqrt{\mathbb{E}_{p_t}\!\|\delta_t(x_t)\|^4}.
% \end{align}
% By Tweedie's formula, $\nabla\log p_t(x_t)=-\gamma_t^{-1}\,\mathbb{E}[z\mid x_t]$.
% Applying conditional Jensen twice
% ($\|\mathbb{E}[z\mid x_t]\|^2\le\mathbb{E}[\|z\|^2\mid x_t]$ and then
% $(\mathbb{E}[\|z\|^2\mid x_t])^2\le\mathbb{E}[\|z\|^4\mid x_t]$),
% \begin{align}
%     \mathbb{E}_{p_t}\!\|\nabla\log p_t(x_t)\|^4
%     =\frac{1}{\gamma_t^4}\mathbb{E}_{p_t}\!\|\mathbb{E}[z\mid x_t]\|^4
%     \le\frac{1}{\gamma_t^4}\mathbb{E}\|z\|^4=\frac{d(d+2)}{\gamma_t^4}.
% \end{align}
% By the Target Score Identity \citep{debortoli2024targetscorematching}, $\nabla\log p_t(x_t)=\alpha_t^{-1}\mathbb{E}[\nabla\log p_1(x_1)|x_t]$. Applying the Jensen's Inequality with \Cref{ass:bounded-4-moment},
% \begin{align}
%     \mathbb{E}_{p_t}\|\nabla\log p_t(x_t)\|^4=\frac{1}{\alpha_t^4}\mathbb{E}_{p_t}\|\mathbb{E}[\nabla\log p_1(x_1)|x_t]\|^4\leq \frac{1}{\alpha_t^4}\mathbb{E}\|\nabla\log p_1(x_1)\|^4=\frac{1}{\alpha_t^4}J_4(p_1).
% \end{align}
% Combining both bounds and taking square roots, we have
% \begin{align}
%     \sqrt{\mathbb{E}_{p_t}\!\|\nabla\log p_t(x_t)\|^4} \leq \min\biggl(\frac{\sqrt{d(d+2)}}{\gamma_t^2}, \frac{\sqrt{J_4(p_1)}}{\alpha_t^2}\biggr)=G_t.
% \end{align}

% By Assumption~\ref{ass:bounded},
% $\mathbb{E}_{p_t}\!\|\delta_t(x_t)\|^4\le B_t^2\mathbb{E}_{p_t}\!\|\delta_t(x_t)\|^2=B_t^2 e_t^2$,
% so $\sqrt{\mathbb{E}_{p_t}\!\|\delta_t(x_t)\|^4}\le B_t e_t$. Hence
% \begin{align}
%     \mathbb{E}_{p_t}\!\bigl[(\nabla\log p_t(x_t)\cdot\delta_t(x_t))^2\bigr]
%     \;\le\;B_t e_t\,G_t.
% \end{align}
% Substituting both bounds into \eqref{eq:Et-pointwise} gives the claim.
% \end{proof}


% \subsubsection{Error of Likelihood Estimation}
% Recall the estimator $\widetilde{\dd_t\log p_t^v}$ from
% \eqref{eq:dlogpv-dt-estimator}. We turn it into a surrogate log-density by
% integrating it along the learned trajectory $\phi$ (where $x_t=\phi_t(x_0)$,
% $x_0\sim p_0$), matching the exact log-density at the same initial condition:
% \begin{align}
%     \log\tilde p_t^v\bigl(\phi_t(x_0)\bigr)
%     &:=\log p_0(x_0)+\int_0^t\!\widetilde{\dd_s\log p_s^v}\bigl(\phi_s(x_0)\bigr)\,ds,\\
%     \log p_t^v\bigl(\phi_t(x_0)\bigr)
%     &=\log p_0(x_0)+\int_0^t\!\dd_s\log p_s^v\bigl(\phi_s(x_0)\bigr)\,ds .
% \end{align}
% We define the likelihood-estimation error
% $\Phi_t(x_t):=\log\tilde p_t^v(x_t)-\log p_t^v(x_t)$. Since the two
% representations share the initial condition, $\Phi_0\equiv0$ and, subtracting,
% \begin{align}
%     \Phi_t\bigl(\phi_t(x_0)\bigr)
%     =\int_0^t\Bigl(\widetilde{\dd_s\log p_s^v}-\dd_s\log p_s^v\Bigr)\bigl(\phi_s(x_0)\bigr)\,ds
%     =\int_0^t \mathcal{E}_s\bigl(\phi_s(x_0)\bigr)\,ds .
%     \label{eq:Phi-integral-rep}
% \end{align}
% This section bounds $\mathbb{E}_{p_t^v}[\Phi_t(x_t)^2]$; the next section
% propagates it to the importance-sampling error.

% \begin{proposition}[Likelihood-estimation error]\label{prop:phi-bound}
% Under \Cref{ass:subgauss,ass:bounded,ass:hess,ass:bounded-4-moment} and quantities defined in \Cref{app:sec:error-bounds:notation}, suppose the
% density-ratio constant $M_s^*:=\|p_s^v/p_s\|_{L^\infty}$ is finite for
% $s\in[0,t]$ ($M_s^*=1$ when $v=v^*$). Then for every $t\in[0,1]$,
% \begin{align}
%     \mathbb{E}_{p_t^v}\!\bigl[\Phi_t(x_t)^2\bigr]
%     \;\le\; t\int_0^t\! M_s^*\,\mathbb{E}_{p_s}\!\bigl[\mathcal{E}_s(x_s)^2\bigr]\,ds
%     \;\le\; 2t\int_0^t\! M_s^*\,e_s\bigl(d\,S_s+B_s\,G_s\bigr)\,ds.
% \end{align}
% \end{proposition}

% \begin{proof}
% Because $x_t=\phi_t(x_0)$ pushes $p_0$ forward to $p_t^v$, the change of
% variables and the integral representation \eqref{eq:Phi-integral-rep} give
% \begin{align}
%     \mathbb{E}_{p_t^v}\!\bigl[\Phi_t(x_t)^2\bigr]
%     =\mathbb{E}_{p_0}\!\left[\left(\int_0^t\mathcal{E}_s(\phi_s(x_0))\,ds\right)^{\!2}\right]
%     \le t\int_0^t\!\mathbb{E}_{p_0}\!\bigl[\mathcal{E}_s(\phi_s(x_0))^2\bigr]\,ds
%     = t\int_0^t\!\mathbb{E}_{p_s^v}\!\bigl[\mathcal{E}_s(x_s)^2\bigr]\,ds,
% \end{align}
% where the inequality is Cauchy--Schwarz in $s$ (Jensen on $[0,t]$) and the last
% equality again uses the pushforward $\phi_s{}_\#p_0=p_s^v$. Transferring each
% inner expectation from $p_s^v$ to $p_s$,
% \begin{align}
%     \mathbb{E}_{p_s^v}\!\bigl[\mathcal{E}_s(x_s)^2\bigr]
%     =\int \frac{p_s^v}{p_s}\,\mathcal{E}_s^2\,p_s\,dx
%     \le M_s^*\,\mathbb{E}_{p_s}\!\bigl[\mathcal{E}_s(x_s)^2\bigr],
% \end{align}
% which proves the first inequality. The second follows by inserting
% \Cref{lem:Et-bound}, $\mathbb{E}_{p_s}[\mathcal{E}_s^2]\le 2e_s(d\,S_s+B_sG_s)$.
% \end{proof}

% \subsubsection{Error of Importance Sampling}
% For a test function $h:\mathbb{R}^d\to\mathbb{R}^k$ we wish to estimate
% \begin{align}
%     H_t:=\mathbb{E}_{p_t}\!\bigl[h(x_t)\bigr]
%     =\mathbb{E}_{p_t^v}\!\left[\frac{p_t(x_t)}{p_t^v(x_t)}\,h(x_t)\right]
% \end{align}
% using samples from the learned flow. Since $p_t^v$ is intractable, we replace it
% by the surrogate $\tilde p_t^v$ of the previous section, giving the estimand
% \begin{align}
%     \tilde H_t:=\mathbb{E}_{p_t^v}\!\left[\frac{p_t(x_t)}{\tilde p_t^v(x_t)}\,h(x_t)\right].
% \end{align}
% With $\Phi_t=\log\tilde p_t^v-\log p_t^v$ as above, a change of variables gives
% \begin{align}
%     H_t-\tilde H_t
%     =\int p_t(x_t)\,h(x_t)\!\left(1-\frac{p_t^v(x_t)}{\tilde p_t^v(x_t)}\right)\!dx_t
%     =\mathbb{E}_{p_t}\!\bigl[h(x_t)\,\bigl(1-e^{-\Phi_t(x_t)}\bigr)\bigr],
% \end{align}
% so by Cauchy--Schwarz in $L^2(p_t)$,
% \begin{align}
%     \|H_t-\tilde H_t\|
%     \le\sqrt{\mathbb{E}_{p_t}\!\|h(x_t)\|^2}\,
%        \sqrt{\mathbb{E}_{p_t}\!\bigl[(1-e^{-\Phi_t(x_t)})^2\bigr]}.
%     \label{eq:IS-CS-1}
% \end{align}
% The mean value theorem gives $1-e^{-u}=u\,e^{-\xi}$ for some $\xi$ between $0$ and
% $u$, hence $|1-e^{-u}|\le|u|\,e^{\max(-u,0)}$. Squaring and writing
% $\kappa_t:=\|e^{\max(-\Phi_t,\,0)}\|_{L^\infty(p_t)}$,
% \begin{align}
%     \mathbb{E}_{p_t}\!\bigl[(1-e^{-\Phi_t(x_t)})^2\bigr]
%     \le\mathbb{E}_{p_t}\!\bigl[\Phi_t(x_t)^2\,e^{2\max(-\Phi_t(x_t),0)}\bigr]
%     \le\kappa_t^2\,\mathbb{E}_{p_t}\!\bigl[\Phi_t(x_t)^2\bigr].
%     \label{eq:IS-CS-2}
% \end{align}
% The integral representation \eqref{eq:Phi-integral-rep} controls $\Phi_t$ along
% the learned flow, i.e.\ under $p_t^v$; we therefore transfer the remaining
% expectation from $p_t$ to $p_t^v$ using $M_t:=\|p_t/p_t^v\|_{L^\infty}$
% ($M_t=1$ when $v=v^*$):
% \begin{align}
%     \mathbb{E}_{p_t}\!\bigl[\Phi_t(x_t)^2\bigr]
%     \le M_t\,\mathbb{E}_{p_t^v}\!\bigl[\Phi_t(x_t)^2\bigr].
%     \label{eq:phi-transfer}
% \end{align}
% Applying \Cref{prop:phi-bound} to the right-hand side and combining with
% \eqref{eq:IS-CS-1}--\eqref{eq:IS-CS-2} yields the main result.

% \begin{theorem}[Importance-sampling error]\label{thm:IS}
%     Under \Cref{ass:subgauss,ass:bounded,ass:hess,ass:bounded-4-moment} and with
%     $\kappa_t,M_t,M_s^*<\infty$, for every $t\in[0,1]$,
%     \begin{align}
%         \|H_t-\tilde H_t\|
%         \;\le\;
%         \sqrt{\mathbb{E}_{p_t}\!\|h(x_t)\|^2}\;\kappa_t\sqrt{M_t}\,
%         \sqrt{2t\int_0^t\! M_s^*\,e_s\!\left(d\,S_s+B_s
%         G_s\right)\,ds}.
%     \end{align}
%     For equilibrium sampling from $p_1$ ($t=1$),
%     \begin{align}
%         \|H_1-\tilde H_1\|
%         \;\le\;
%         \sqrt{\mathbb{E}_{p_1}\!\|h(x_1)\|^2}\;\kappa_1\sqrt{M_1}\,
%         \sqrt{2\int_0^1\! M_s^*\,e_s\!\left(d\,S_s+B_sG_s\right)\,ds}.
%     \end{align}
% \end{theorem}

% \begin{remark}
%     The constants $\kappa_t,M_t,M_s^*$ all reduce to $1$ in the well-specified
%     limit $v\to v^*$, where $e_s\equiv0$ and both bounds vanish. They isolate the
%     deviation of the sampling measure $p_t^v$ from the target $p_t$:
%     \Cref{prop:phi-bound} controls the \emph{accumulated} likelihood error along
%     the flow via $M_s^*$, while the extra factor $M_t$ in \eqref{eq:phi-transfer}
%     converts that path-level guarantee into a target-level one. The local fidelity
%     of the estimator itself is carried by \Cref{lem:Et-bound}.
% \end{remark}
