# Supplementary material for: Few-Step Boltzmann Generators via Scalable Likelihood Flow Maps
Source: arXiv:2606.29110 source file (2026-11-03)
Supplement: Supplementary file 5 [file molecular_and_se3.tex]

% \section{Experimental Details for $n$-body systems}

% In this section, we detail the experimental design for modeling $n$-body systems, such as molecules. A sample from an $n$-body system consists of $n$ particles and exhibits symmetries under the $\mathrm{E}(3)$ or $\mathrm{O}(3)$ group. For a single particle's coordinate $a \in \mathbb{R}^3$ and a rotation matrix $R \in \mathrm{O}(3)$, a function $g: \mathbb{R}^3 \rightarrow \mathbb{R}^3$ is \emph{rotationally equivariant} if
% \begin{align}
%     g(Ra) = Rg(a),
% \end{align}
% and a function $h: \mathbb{R}^3 \rightarrow \mathbb{R}$ is \emph{rotationally invariant} if
% \begin{align}
%     h(Ra) = h(a).
% \end{align}

% Let $x \in \mathbb{R}^{3n}$ represent the flattened spatial coordinates of the $n$-body system. We define the global rotation operator as a block-diagonal matrix $R_n = I_n \otimes R \in \mathbb{R}^{3n \times 3n}$, where $\otimes$ denotes the Kronecker product. Let $v: \mathbb{R}^{3n} \rightarrow \mathbb{R}^{3n}$ be an $\mathrm{O}(3)$-equivariant velocity field, satisfying:
% \begin{align}
%     v(R_nx) = R_nv(x).
% \end{align}

% Let $J_v(x) := \nabla_x v(x) \in \mathbb{R}^{3n \times 3n}$ denote the Jacobian of $v$ evaluated at $x$. By applying the chain rule to the left-hand side and the linearity of $R_n$ to the right-hand side of the equivariance condition, we obtain:
% \begin{align}
%     J_v(R_nx)R_n = R_nJ_v(x).
% \end{align}
% Right-multiplying by $R_n^{-1} = R_n^\top$, we derive the transformation rule for the Jacobian:
% \begin{align}
%     J_v(R_nx) = R_nJ_v(x)R_n^\top.
% \end{align}
% This demonstrates that $J_v(x)$ transforms identically to a Cartesian rank-2 tensor under rotation. Consequently, its trace and diagonal entries transform as:
% \begin{align}
%     \mathrm{tr}(J_v(R_nx)) &= \mathrm{tr}\bigl(R_nJ_v(x)R_n^\top\bigr) = \mathrm{tr}\bigl(R_n^\top R_nJ_v(x)\bigr) = \mathrm{tr}(J_v(x)) \\
%     \mathrm{diag}(J_v(R_nx)) &= \mathrm{diag}\bigl(R_nJ_v(x)R_n^\top\bigr)
% \end{align}

% % TODO: Consider inserting a figure here demonstrating a 3x3 rank-2 tensor decomposition into trace, antisymmetric, and symmetric traceless components.

% Thus, the trace of the Jacobian (the divergence) is a purely rotationally invariant scalar ($l=0$), while the diagonal of the Jacobian relies on the full rank-2 tensor projection, containing both $l=0$ and symmetric-traceless $l=2$ components.

% \subsection{Implication to Neural Network Architecture}
% In practice, the velocity $v$ is parameterized by an equivariant graph neural network (EGNN). Given invariant node features $h$ and equivariant coordinates $x$, the network outputs updated invariant features $h'$ and equivariant vector updates $x'$, i.e.
% \begin{align}
%     x',h'\leftarrow \mathrm{EGNN}(x,h).
% \end{align}

% \paragraph{Predicting Scalar Divergence.} To predict the standard divergence (the trace of the Jacobian), we utilize the updated invariant node features $h'$ of the EGNN. Because the trace is strictly $l=0$, we safely feed $h'$ into a standard Multi-Layer Perceptron (MLP) to obtain a scalar prediction per node:
% \begin{align}
%     \hat{J}_v(x) \leftarrow \mathrm{MLP}(h').
% \end{align}

% \paragraph{Predicting Vectorized Divergence.} The diagonal of the Jacobian is not a standard equivariant vector; it cannot be approximated by an $l=1$ output. To correctly recover it, we must synthesize a rank-2 tensor. If $u, w \in \mathbb{R}^3$ are two $l=1$ equivariant vectors, their outer product $u w^\top$ forms a valid rank-2 tensor that obeys the $R(\cdot)R^\top$ transformation rule. 

% To expressively parameterize this, we predict $K$ pairs of equivariant vectors $U, W \in \mathbb{R}^{n \times 3 \times K}$ per node. First, for each directed edge $(i, j)$, we compute the normalized equivariant relative coordinate differences $\hat{r}_{ij} = (x_i - x_j) / (\|x_i - x_j\| + c)$ alongside the invariant edge attributes $h_{ij}$. We process these invariant attributes through a Multi-Layer Perceptron (MLP) to predict $2K$ rotationally invariant ($l=0$) scalar weights per edge:
% \begin{align}
%     s_{ij} = \mathrm{MLP}(h_{ij}) \in \mathbb{R}^{2K}.
% \end{align}
% These scalars are then multiplied by the $l=1$ directional vectors $\hat{r}_{ij}$ to construct $2K$ equivariant edge vectors. These are subsequently aggregated over the local neighborhood $\mathcal{N}(i)$ of each node $i$ (e.g., via mean pooling) to form node-level equivariant features:
% \begin{align}
%     \vec{V}_i = \frac{1}{|\mathcal{N}(i)|} \sum_{j \in \mathcal{N}(i)} s_{ij} \otimes \hat{r}_{ij} \in \mathbb{R}^{3 \times 2K}.
% \end{align}
% We split these $2K$ vector channels into two equal sets to form our matrices $U$ and $W$. We then compute the diagonal of their combined tensor product:
% \begin{align}
%     \widehat{\mathrm{diag}(J_v)} \leftarrow \sum_{k=1}^K U_{:,:,k} \odot W_{:,:,k},
% \end{align}
% where $\odot$ denotes element-wise multiplication. This guarantees that the regression objective respects the fundamental $\mathrm{O}(3)$ geometry of the Jacobian diagonal. 

% Crucially, the hyperparameter $K$ must be constrained such that $K \ge 3$. Because the tensor product $\sum_{k=1}^K \vec{u}^{(k)} (\vec{w}^{(k)})^\top$ represents the sum of $K$ rank-1 outer products, the rank of the resulting predicted Jacobian is mathematically bounded by $K$. In three-dimensional space, the true physical Jacobian $J_v \in \mathbb{R}^{3 \times 3}$ describes stretching and shearing across all three spatial dimensions independently and is generally full-rank. Therefore, $K \ge 3$ is strictly required to ensure the network possesses the sufficient degrees of freedom to span the entire space of possible 3D Jacobians.
